# Supplementary material for: GeoGround: A Unified Large Vision-Language Model for Remote Sensing Visual Grounding
Source: arXiv:2411.11904 source file (2025-05-10)
Supplement: Supplementary file 1 [file X_suppl.tex]

\clearpage
\setcounter{page}{1}
\setcounter{section}{0} 
\maketitlesupplementary

\section{Additional Visual Grounding Signal Details}

\subsection{Type of Signals used in VLMs.}

Tab. \ref{tab:loc_signal} summarizes several visual grounding signals currently employed in the VLM domain, all of which use the signal textualization paradigm to convert visual grounding tasks into text generation tasks. To the best of our knowledge, we are the first to convert masks of RS objects into text sequences successfully.

\begin{table}[h]
\vspace{-0.3cm}
\resizebox{\columnwidth}{!}{
	% \scalebox{0.8}[0.8]{
  \centering
  \setlength{\tabcolsep}{2pt}
  \begin{tabular}{lcccc}
    \toprule
    % \rowcolor{mygray}
     
    Model & Signal & Density & Resolution &Text Length \\
    \midrule
    Kosmos-2~\cite{peng2023kosmos} & HBB & Sparse & 1/32 & 2 tokens    \\
    Shikra~\cite{chen2023shikra} & HBB & Sparse & 1/1000 & 4 numbers     \\
    GeoChat~\cite{kuckreja2024geochat} & OBB & Medium & 1/100 & 5 numbers     \\
    EarthGPT~\cite{zhang2024earthgpt} & Polygon & Medium & 1/100 & 8 numbers    \\
    Text4Seg~\cite{anonymous2024textseg} & Mask & Dense & 1/N & N$\times$N phases     \\
    \rowcolor{myblue}GeoGround & Mask & Dense & 1/N & N$\times$N numbers     \\
    \bottomrule
  \end{tabular}}
  \vspace{-0.2cm}
    \caption{Comparison of different signals used in VLMs.}
    \label{tab:loc_signal}
\vspace{-0.2cm}
\end{table}

\subsection{Format of HBB Signals.}

Tab. \ref{tab:token_cnt} presents the numerical ranges and representation precision of several common HBB encoding formats in current grounded VLMs. Additionally, we calculated the number of tokens required by the LLaVA tokenizer to encode a single object using these formats. Format \#1, adopted by GeoChat~\cite{kuckreja2024geochat}, requires more tokens than \#2 for the same precision. Since the tokenizer requires more tokens to encode decimal values, Format \#3, which normalizes coordinates to 1 and retains three decimal places, results in the highest token count. We recommend using \#4 or \#5, corresponding to the InternVL~\cite{chen2023internvl} and Qwen-VL~\cite{bai2023qwen} formats, respectively, as they offer greater precision while requiring fewer tokens. Reducing the number of tokens needed to encode a single object not only lowers the training cost for VLMs but also accelerates inference.  Ultimately, we selected \#4 as the default HBB format for GeoGround.

\begin{table}[h]
\vspace{-0.3cm}
\resizebox{\columnwidth}{!}{
	% \scalebox{0.8}[0.8]{
  \centering
  \setlength{\tabcolsep}{3pt}
  \begin{tabular}{ccccc}
    \toprule
    % \rowcolor{mygray}

    \# & Range & Precision & Format & \#Token \\
    \midrule
    1 & [0,100) & 100 &  $\{\textless x_1 \textgreater\textless y_1 \textgreater\textless x_2 \textgreater\textless y_2 \textgreater\}$ & 12$\sim$20   \\
    2 & [0, 100) & 100 & $[x_1,y_1,x_2,y_2]$ & 10$\sim$14   \\
    3 & [0,1) & 1000 & $[x_1,y_1,x_2,y_2]$ & 18$\sim$26   \\
    \rowcolor{mylightblue}4 & [0, 1000) & 1000 & $[x_1,y_1,x_2,y_2]$ & 10$\sim$18   \\
    \rowcolor{myblue}5 & [0, 1000) & 1000 &  $(x_1,y_1),(x_2,y_2)$ & 10$\sim$18   \\
    \bottomrule
  \end{tabular}}
    \caption{Token counts required for encoding several HBB formats using LLaVA model's tokenizer.}
    \label{tab:token_cnt}
\end{table}

\subsection{Resolution of Signals.}

Fig. \ref{fig:disappear_rate} compares the disappearance rates of objects across 5 remote sensing visual grounding datasets when different quantization resolutions are applied. It can be observed that the datasets, ranked by the proportion of small targets from highest to lowest at a quantization resolution of 16, are RSVG, AVVG, GeoChat, DIOR-RSVG, and VRSBench. This also explains why the VLM scores are relatively low on the RSVG and AVVG datasets. When the quantization resolution is set to 32, the object disappearance rate remains below 20\% for all datasets. Thus, Matrix4Seg achieves satisfactory performance when the resolution is set to 32. At a quantization resolution of 100, GeoChat still has a disappearance rate of 12.65\%, indicating the presence of some very small targets in the GeoChat dataset.

\begin{figure}[!t]
% \vspace{-0.2cm}
	\begin{center}             % figure uses center environment
        \includegraphics[width=1\linewidth]{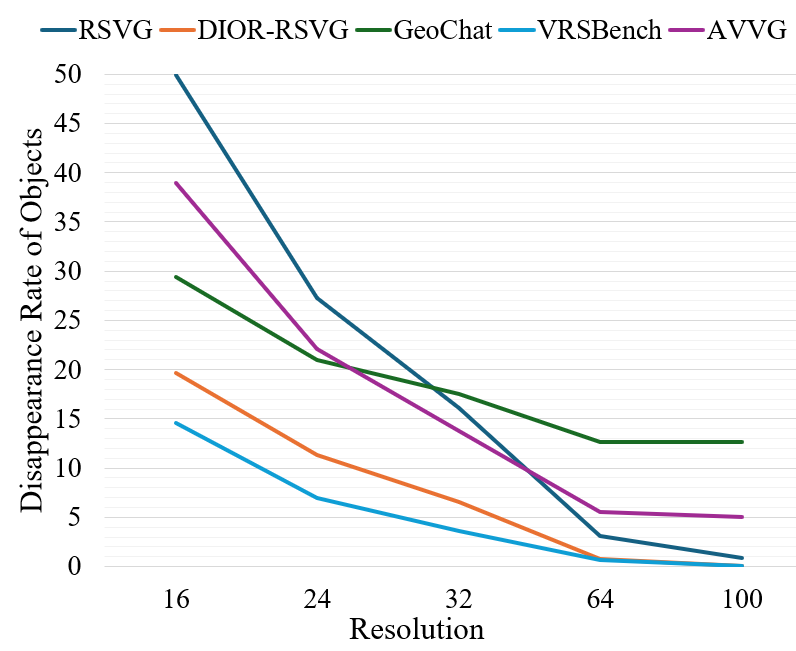}
    \end{center}
    \vspace{-0.5cm}
    \caption{Disappearance rate of objects in masks after resizing to N$\times$N dimensions. The higher the proportion of small objects in the dataset, the greater the disappearance rate.}
    \label{fig:disappear_rate}          % label is always after caption
    \vspace{-0.3cm}
\end{figure}

\section{Additional Data Details}

\subsection{Mask Generation.}

The released refGeo dataset contains manually annotated HBBs or OBBs. However, the masks used in the experiments are generated through an automated method, and thus their quality cannot be fully guaranteed. Although we set a score threshold, errors in the masks still occur. Interestingly, despite the noise in these mask data, they still validate the effectiveness of the hybrid supervision training proposed in this paper. In future work, we plan to manually refine these automatically generated masks in refGeo to provide more accurate referring expression segmentation samples for training.

\subsection{Creation of AVVG.}

Existing open-source RS datasets~\citep{xia2018dota,li2020object} often lack sensor metadata and provide limited target attributes. Consequently, these datasets can only support the formulation of simple visual grounding problems, such as  locating a object in the upper-left corner of an image. To develop a spatially aware remote sensing dataset, we use unmanned aerial vehicles to collect data from scratch. This approach ensures comprehensive access to sensor parameters, allowing inversion of the three-dimensional coordinates of image targets based on imaging geometry principles. Data collection is divided into two parts: aerial imagery and ground video.

\paragraph{Aerial Imagery.} 
All aerial images in AVVG are collected with a small UAV platform, DJI Mini3, between 10-16 September 2023, in Shanghai. The dataset consists of 4K high-resolution RS images from 11 distinct scenes, captured at 9 different above-ground levels and 3 pitch angles. This implies that these RS images possess different spatial resolutions and perspectives. In addition, the collected images cover a variety of weather scenarios, such as sunny, cloudy, and rainy days, along with different lighting conditions.

\paragraph{Ground Video.} We record ground videos from the same areas to facilitate accurate annotation of vehicle brands and models. Specifically, we select time slots with relatively low vehicular mobility, avoiding rush hours and meal times. Additionally, to mitigate the vehicle mismatch between drone images and ground videos caused by vehicle entry and exit, we capture two sets of ground videos before and after the drone captures aerial photos. This ensures that vehicles entering or exiting the scene halfway through the capture are recorded in the videos. However, there are instances where vehicles pass through the scene briefly, leading to cases where they are not captured in either video. In such situations, we mask these vehicles with a black mask in the images to ensure that all visible vehicles have fully known attributes. Due to privacy concerns, ground videos will not be released. 

\paragraph{Derivation of Coordinate System Transformation.}

\begin{figure}[h]
% \vspace{-0.2cm}
	\begin{center}             % figure uses center environment
\includegraphics[width=1\linewidth]{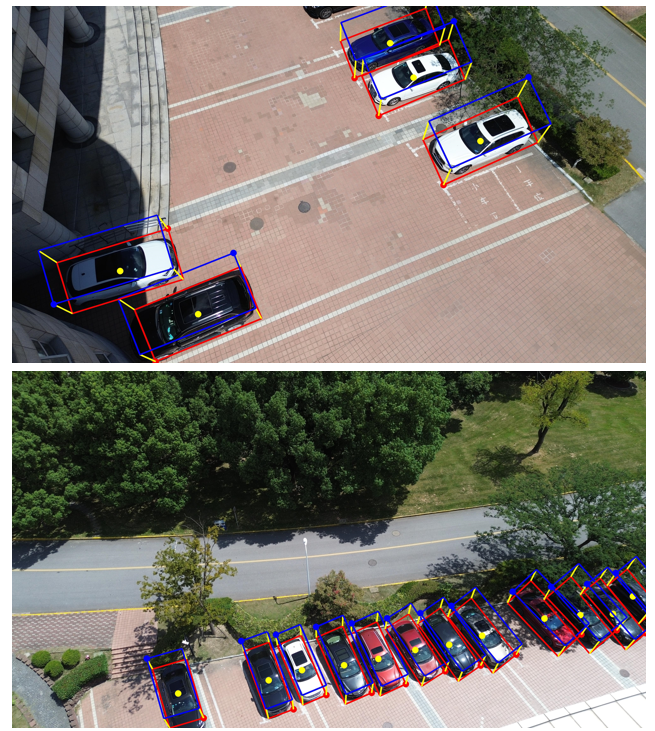}
    \end{center}
    \vspace{-0.5cm}
    \caption{Illustration of the 3D bounding box are obtained by Coordinate System Transformation.}
    \label{fig:3d_box}          % label is always after caption
    \vspace{-0.3cm}
\end{figure}

The transformation between the pixel coordinate system and the image coordinate system can be represented by an affine matrix, as follows:
\begin{equation}
\begin{split}
\left[ \begin{array}{c}
	x_P\\
	y_P\\
	1\\
\end{array} \right] =\left[ \begin{matrix}
	\frac{1}{p}&		0&		\frac{w}{2}\\
	0&		\frac{1}{p}&		\frac{h}{2}\\
	0&		0&		1\\
\end{matrix} \right] \left[ \begin{array}{c}
	x_I\\
	y_I\\
	1\\
\end{array} \right] 
\end{split}
\label{Equ:1}
\end{equation}
where $p$ represents the pixel size of the sensor. $\frac{w}{2}$ and $\frac{h}{2}$ denote the origin offsets, with the origin of the image coordinate system typically located at the image's top-left corner. Given the pixel coordinates of a certain point, its corresponding image coordinates can be calculated as follows:
\begin{equation}
\begin{split}
\begin{cases}
x_I = (x_P - w/2) \cdot p \\
y_I = (y_P - h/2) \cdot p
\end{cases}
\end{split}
\label{Equ:1}
\end{equation}

The transformation from the camera coordinate system to the image coordinate system is a conversion from three-dimensional to two-dimensional coordinates. Assuming the focal length of the camera is $f$, then we have
\begin{equation}
\begin{split}
z_c\left[ \begin{array}{c}
	x_I\\
	y_I\\
	1\\
\end{array} \right] =\left[ \begin{matrix}
	f&		0&		0&		0\\
	0&		f&		0&		0\\
	0&		0&		1&		0\\
\end{matrix} \right] \left[ \begin{array}{c}
	x_C\\
	y_C\\
	z_C\\
	1\\
\end{array} \right] 
\end{split}
\label{Equ:2}
\end{equation}
where $z_C$ denotes the depth of the point, which can be obtained by a depth camera (binocular or structured light). Because the drone camera we are using cannot provide depth information, we need to find another way.

When the ground satisfies the ground plane assumption, given the AGL of the drone and the pitch angle of the camera, the ground plane equation in the camera coordinate system is as follows:
\begin{equation}
\begin{split}
-\cos{\theta} \cdot Y_C - \sin{\theta} \cdot Z_C + H = 0 
\end{split}
\label{Equ:3}
\end{equation}

The equation of the line connecting the camera origin to the projection point on the pixel plane in the camera coordinate system is given by:
\begin{equation}
\begin{split}
\begin{cases}
X_C = x_I \cdot t \\
Y_C = y_I \cdot t\\
Z_C = f \cdot t
\end{cases}
\end{split}
\label{Equ:4}
\end{equation}

Substituting the line equation into the ground plane equation yields:
\begin{equation}
\begin{split}
t = \frac{H}{y_I\cos{\theta} + f\sin{\theta} }
\end{split}
\label{Equ:5}
\end{equation}

Substituting $t$ back into the line equation yields:
\begin{equation}
(\frac{x_I  H}{y_I\cos{\theta} + f\sin{\theta}}, \frac{y_I  H}{y_I\cos{\theta} + f\sin{\theta}}, \frac{f  H}{y_I\cos{\theta} + f\sin{\theta}})
\label{Equ:5}
\end{equation}

Fig. \ref{fig:3d_box} visualizes the 3D bounding box of a vehicle. The implementation process is as follows: First, the 3D coordinates of the vehicle's center point are calculated in the camera coordinate system. Then, based on the orientation information and the vehicle’s length, width, and height, the 3D coordinates of its eight corner points are computed. Finally, these points in the 3D coordinate system are projected back into the 2D-pixel coordinate system. The visualization results further validate the correctness of this coordinate transformation. With the 3D bounding box of each vehicle available, we can formulate visual grounding problems that require the model to have spatial reasoning abilities to solve. For example, which vehicle is the farthest from the camera? Which vehicle has the highest height? 

To preserve the spatial mapping between camera coordinates and pixel coordinates, we refrained from cropping the 4K images to increase the dataset size, as is commonly done in most remote sensing datasets. Since the problems involve fine-grained attributes of the vehicles, we used the HBB coordinates of the object as the answers to these spatial grounding tasks, rather than the 3D bounding box, to control the difficulty and prevent the tasks from becoming excessively challenging.

\paragraph{Generalized REC Benchmark.}

The generalized referring expression comprehension benchmark built using AVVG includes AP@0.5 scores for three fine-grained vehicle attributes. The specific categories for each attribute are listed as follows: \textbf{Color (13)}: golden, brown, orange, silver, gray, blue, white, red, black, pink, green, yellow, purple. \textbf{Type (10)}: compact, suv, mid-size, subcompact, mpv, sports, full-size, crossover, sedan, micro-size. \textbf{Brand (52)}: skoda, buick, audi, toyota, tesla, volkswagen, mercedes-benz, nio, chevrolet, mazda, hyundai, lexus, honda, bmw, ora, geely, byd, jeep, volvo, renault, roewe, ford, nissan, infiniti, peugeot, cadillac, rising, aito, xpeng, haval, lynk\&co, mini, citroen, riich, leap, wey, ideal, changan, harvard, denza, chery, kia, porsche, mg, beijing, smart, baojun, aion, wuling, vgv, hongqi, lexus, lincoln.

\section{Additional Implementation Details}
% \label{sec:rationale}

We employ the LLaVA framework to train LLaVA-1.5 and GeoChat, while the SWIFT~\cite{zhao2024swift} framework is used to train the Qwen-VL model.  The main experiments cover 3 types of connectors, including MLP (LLaVA-1.5, GeoChat), Pixel Shuffle +
MLP (InternVL2) and Cross-attention (Qwen-VL). In addition, the selected VLMs have different input image resolutions: fixed 336$\times$336 for LLaVA-1.5, fixed 448$\times$448 for Qwen-VL, fixed 504$\times$504 for GeoChat, and dynamic input resolution for InternVL2 and Qwen2-VL. 

\subsection{Details of Training Hyper-parameters.}

Tab. \ref{tab:params} presents the training hyperparameters used to train the GeoGround. We adhere primarily to the same settings as GeoChat~\cite{kuckreja2024geochat}, and these parameters are also consistently applied in other fine-tuned VLMs in this paper. However, we observed that two novel VLMs that support dynamic resolution images, InternVL2~\cite{chen2023internvl} and Qwen2-VL~\cite{wang2024qwen2}, struggled to achieve satisfactory fine-tuning results with the same set of parameters. Unfortunately, we have not yet identified satisfactory training parameters for them.

\begin{table}[!t]
\vspace{-0.3cm}
\resizebox{\columnwidth}{!}{
	% \scalebox{0.8}[0.8]{
  \centering
  \setlength{\tabcolsep}{3pt}
    \begin{tabular}{c|l|c}
        \hline
                                   & Param Name & Value \\ \hline
        \multirow{7}{*}{Optimizer} & Type  & AdamW  \\
                                   & Learning rate   & 2e-4 \\
                                   & Weight decay  & 0.0 \\
                                   & $(\beta_1, \beta_2)$  & (0.9, 0.95) \\
                                   & Gradient norm clip    & 1.0 \\ 
                                   & Scheduler & Linearly decay \\
                                   & Warmup ratio & 0.03 \\  \hline
        \multirow{4}{*}{LoRA}      & Rank                  & 64 \\
                                   & Alpha ($\alpha$)      &  16 \\
                                   & Dropout & 0.05 \\
                                   & Module                &  Linear layers of connector and LLMs \\ \hline
        \multirow{5}{*}{Training}  & Trainable \#Params.   &  About 2\% of the LLM (7B $\rightarrow$ 160M)\\
                                   & Numerical precision   &  FP16 \\
                                   & Global batch size            &  128 \\
                                   & Total epochs          &  5 \\
                                   & GPUs                  & V100(32G) $\times$ 8 \\
                                   \hline
    \end{tabular}}
    \caption{Hyper-parameters and training settings for GeoGround.}
    \label{tab:params}
\end{table}

\subsection{Details of Object Detection Training Samples.}

We construct a fine-grained vehicle object detection benchmark leveraging the metadata from the \texttt{test} split of our proposed AVVG dataset. Additionally, to assess performance on remote sensing object detection, we create a dataset consisting of 200k samples by combining data from DOTA~\cite{xia2018dota}, DIOR~\cite{li2020object}, FAIR1M~\cite{sun2022fair1m}, and the \texttt{train} split of AVVG. Specifically, we first cropped the original images from the FAIR1M~ and DOTA datasets into 512$\times$512 patches, while retaining the original image sizes for the DIOR and AVVG datasets. We then used the object detection annotations from these datasets to generate training samples, where queries were formulated based on the categories present in each image. Specifically, if an image contains objects from three categories, we constructed three image-text sample pairs accordingly. These data are used to enhance GeoGround's basic visual perception capabilities.

\subsection{Implementation of Mask Refiner.}

\begin{figure}[!t]
% \vspace{-0.2cm}
	\begin{center}             % figure uses center environment
\includegraphics[width=1\linewidth]{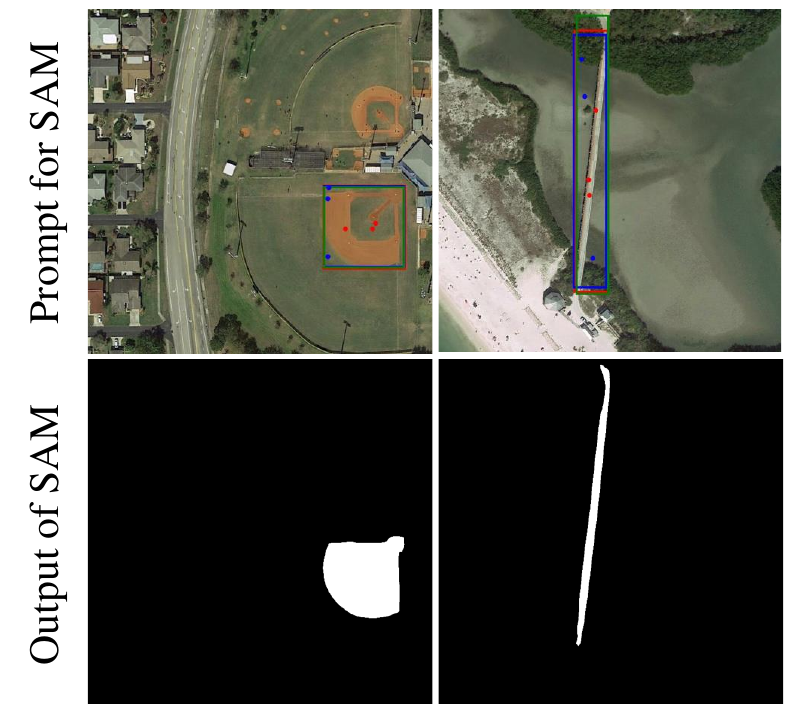}
    \end{center}
    \vspace{-0.5cm}
    \caption{Illustration of the process of refining masks using the SAM. The red and blue dots represent the sampled positive and negative data points. The red, blue, and green bounding boxes represent the ground truth (GT), the GeoGround prediction, and the bounding box of the mask output by SAM, respectively.}
    \label{fig:sam_prompt}          % label is always after caption
    \vspace{-0.3cm}
\end{figure}

Due to resolution limitations, the proposed Matrix4Seg currently struggles to segment particularly small targets. To address this issue, we can simply refine the output masks using SAM to obtain more accurate masks. Specifically, we resize the binary matrix output from the model to match the dimensions of the image, generating a coarse mask. We then sample 3 positive points and 3 negative points from the mask. The sampling region for the positive points is the intersection between the coarse mask and the predicted HBB, while the sampling region for the negative points is the difference between the coarse mask and the predicted HBB. Subsequently, the positive and negative points, along with the predicted HBB, are used as prompts and input into SAM. If no positive or negative sample points are available, only the predicted HBB is used as the prompt for SAM. Since SAM is training-free, it can be regarded as a post-processing method. As shown in Tab. \ref{tab:ae_2}, the precision of the masks can be further improved after refinement.

\subsection{Visual Instruction Templates}

Fig. \ref{fig:template}  lists all the instruction templates used during the training of GeoGround. During training, a query is randomly selected from a set of five for each iteration.

\section{Additional Quantitative Results}

\subsection{More Results on REC.}

\begin{table}[!t]
\vspace{-0.3cm}
\resizebox{\columnwidth}{!}{
	% \scalebox{0.8}[0.8]{
  \centering
  \setlength{\tabcolsep}{2pt}
  \begin{tabular}{cccccc}
    \toprule
    % \rowcolor{mygray}

    DIOR-RSVG & RSVG & GeoChat & VRSBench & AVVG & Acc@0.5 \\
    \midrule
    \icoyes & \icono & \icono  & \icono & \icono & 58.74   \\
    \icoyes & \icoyes & \icono  & \icono & \icono & 59.84   \\
    \icoyes & \icoyes & \icoyes  & \icono & \icono & 63.34   \\
    \icoyes & \icoyes & \icoyes  & \icoyes & \icono & 65.91   \\
    \rowcolor{myblue}\icoyes & \icoyes & \icoyes  & \icoyes & \icoyes & \textbf{65.98}   \\
    \bottomrule
  \end{tabular}}
  \vspace{-0.2cm}
    \caption{Influence of varying training sample sizes on the LLaVA model's REC performance on DIOR-RSVG test set.}
    \label{tab:ae_1}
    \vspace{0.2cm}
\end{table}

Tab. \ref{tab:ae_1} shows that as more supervised fine-tuning samples are added to the training set, the Acc@0.5 metric, computed using HBBs on the DIOR-RSVG test set, exhibits a continuous upward trend for the LLaVA-1.5-7B model. This indicates that the scaling law remains effective, suggesting that further increasing the number of visual grounding samples in the RS domain is still a promising avenue. 

\begin{table}[!t]
\vspace{-0.3cm}
\resizebox{\columnwidth}{!}{
	% \scalebox{0.8}[0.8]{
  \centering
  \setlength{\tabcolsep}{9pt}
  \begin{tabular}{ccccc}
    \toprule
    % \rowcolor{mygray}
    DIOR & DOTA & FAIR1M & AVVG & Acc@0.5 \\
    \midrule
    \icono & \icono & \icono  & \icono & 58.74   \\
    \icoyes & \icono & \icono  & \icono &  59.70   \\
    \icoyes & \icoyes & \icono  & \icono & 72.61   \\
    \icoyes & \icoyes & \icoyes  & \icono & \textbf{73.59}   \\
    \rowcolor{myblue}\icoyes & \icoyes & \icoyes  & \icoyes & 73.43   \\
    \bottomrule
  \end{tabular}}
    \caption{Influence of varying object detection sample sizes on the LLaVA model's REC performance for the DIOR-RSVG test set.}
    \label{tab:ae_5}
\end{table}

\begin{table}[!t]
\vspace{-0.3cm}
\resizebox{\columnwidth}{!}{
	% \scalebox{0.8}[0.8]{
  \centering
  \setlength{\tabcolsep}{6pt}
  \begin{tabular}{ccccc}
    \toprule
    % \rowcolor{mygray}
    AVVG & DIOR & DOTA & FAIR1M  & Overall AP@0.5 \\
    \midrule
    \icoyes & \icono & \icono  & \icono &  1.04   \\
    \icoyes & \icoyes & \icono  & \icono & 3.11   \\
    \icoyes & \icoyes & \icoyes  & \icono & 4.05   \\
    \rowcolor{myblue}\icoyes & \icoyes & \icoyes  & \icoyes & \textbf{4.95}   \\
    \bottomrule
  \end{tabular}}
    \caption{Influence of varying training sample sizes on the LLaVA model's Generalized REC performance for the AVVG test set.}
    \label{tab:ae_8}
\end{table}

Furthermore, we conducted an in-depth investigation into the impact of object detection on the REC task. As shown in Tab. \ref{tab:ae_5}, incorporating object detection samples during training can also improve the REC performance of the model. An interesting observation is that, although DIOR-RSVG is constructed using images from the DIOR dataset for the visual grounding task, incorporating object detection samples from the DIOR dataset only improves the results by approximately 1\%. However, when object detection samples from the DOTA dataset are added, whose images come from a different source, the performance increases by more than 10\%. This indicates that the improvement in the performance of the REC task through object detection is not only due to data leakage. Since the AVVG data set is designed for fine-grained vehicle attribute detection and only contains vehicles as target objects, it does not contribute to the performance improvement in the DIOR-RSVG data set.

% \subsection{More Results on RES.}

% \begin{table}[h]
% % \vspace{0.3cm}
% \resizebox{\columnwidth}{!}{
% 	% \scalebox{0.8}[0.8]{
%   \centering
%   \setlength{\tabcolsep}{2pt}
%   \begin{tabular}{cccccc}
%     \toprule
%     % \rowcolor{mygray}

%     Methods & LISA & PixelLM & NExT-Chat & Text-Mask & Text-Mask+SAM  \\
%     \midrule
%     Image size & 224$^2$ & 448$^2$  & 336$^2$ & 336$^2$ & 336$^2$   \\
%     Time (s) & 3.67 & 6.60 & 6.27 & 4.31 & 6.40 \\
%     \bottomrule
%   \end{tabular}}
%   \vspace{-0.2cm}
%     \caption{Inference time of VLMs on RRSIS-D test set.}
%     \label{tab:ae_ss}
%     \vspace{-0.2cm}
% \end{table}

% Tab. \ref{tab:ae_ss} compares the inference speed of the proposed method with several vision-language models (VLMs) that support the RES task on the RRSIS-D test set. This experiment is conducted on a single V100 GPU. The resolution of the Text-Mask is set to 16. The proposed method achieves the second-fastest inference speed, surpassed only by LISA, and significantly outperforms PixelLM and NExT-Chat when SAM is not used. Even with the addition of SAM as a mask refiner, the inference speed of the proposed method remains competitive.

\subsection{More Results on Generalized REC.}

Tab. \ref{tab:ae_8} shows that adding Generalized REC training samples based on other object detection datasets can also improve the model's performance on AVVG.

\subsection{Inference Time}  

\begin{table}[t]
% \vspace{0.3cm}
\resizebox{\columnwidth}{!}{
	% \scalebox{0.8}[0.8]{
  \centering
  \setlength{\tabcolsep}{2pt}
  \begin{tabular}{cccccc}
    \toprule
    % \rowcolor{mygray}

    Methods & LISA & PixelLM & NExT-Chat &  Text-Mask & Text-Mask+SAM  \\
    \midrule
    Image size & 224$^2$ & 448$^2$  & 336$^2$ & 336$^2$ & 336$^2$   \\
    Time (s) & 3.67 & 6.60 & 6.27 & 4.31 & 6.40 \\
    \bottomrule
  \end{tabular}}
  \vspace{-0.2cm}
    \caption{Inference time of VLMs on RRSIS-D.}
    \label{tab:ae_ss}
    \vspace{-0.4cm}
\end{table}

Tab. \ref{tab:ae_ss} compares the inference speed of the proposed method with several VLMs that support the RES task on the RRSIS-D test set. This experiment is conducted on a single V100 GPU. The resolution of the Text-Mask is set to 16. The proposed method achieves the second-fastest inference speed, surpassed only by LISA, and significantly outperforms PixelLM and NExT-Chat when SAM is not used. Even with the addition of SAM as a mask refiner, the inference speed of the proposed method remains competitive.

\begin{table*}[!t]
\fontsize{9.0pt}{\baselineskip}\selectfont
\linespread{0.9}\selectfont
\begin{mybody}
\textbf{Query for REC:} \\
$[$refer$]$ give me the bounding box of $<$ref$>$\{prompt\}$<$/ref$>$\\
$[$refer$]$ output the bounding box of the $<$ref$>$\{prompt\}$<$/ref$>$ in the image.\\
$[$refer$]$ from this image, provide the bounding box for $<$ref$>$\{prompt\}$<$/ref$>$.\\
$[$refer$]$ please provide the bounding box coordinate of the region this sentence describes: $<$ref$>$\{prompt\}$<$/ref$>$\\
$[$refer$]$ can you locate and provide the bounding box for $<$ref$>$\{prompt\}$<$/ref$>$ in the given image?\\
\textbf{Response:} $<$box$>$\{hbb\}$<$/box$>$\\\\
\textbf{Query for REC with OBB:} \\
$[$refer$]$ give me the oriented bounding box of $<$ref$>$\{prompt\}$<$/ref$>$\\
$[$refer$]$ output the oriented bounding box of the $<$ref$>$\{prompt\}$<$/ref$>$ in the image.\\
$[$refer$]$ from this image, provide the oriented bounding box for $<$ref$>$\{prompt\}$<$/ref$>$.\\
$[$refer$]$ please provide the oriented bounding box coordinate of the region this sentence describes: $<$ref$>$\{prompt\}$<$/ref$>$\\
$[$refer$]$ can you locate and provide the oriented bounding box for $<$ref$>$\{prompt\}$<$/ref$>$ in the given image?\\
\textbf{Response:} $<$obb$>$\{obb\}$<$/obb$>$\\\\
\textbf{Query for RES:} \\
$[$refer$]$ give me the segmentation mask of $<$ref$>$\{prompt\}$<$/ref$>$\\
$[$refer$]$ output the segmentation mask of the $<$ref$>$\{prompt\}$<$/ref$>$ in the image.\\
$[$refer$]$ from this image, provide the segmentation mask for $<$ref$>$\{prompt\}$<$/ref$>$.\\
$[$refer$]$ please provide the segmentation mask of the region this sentence describes: $<$ref$>$\{prompt\}$<$/ref$>$.\\
$[$refer$]$ can you segment the $<$ref$>$\{prompt\}$<$/ref$>$ in the given image?\\
\textbf{Response:} $<$seg$>$\{mask\}$<$/seg$>$\\\\
\textbf{Query for Object Detection:}\\
$[$refer$]$ give me the bounding box of all $<$ref$>$\{prompt\}$<$/ref$>$\\
$[$refer$]$ output the bounding box of all $<$ref$>$\{prompt\}$<$/ref$>$ in the image.\\
$[$refer$]$ from this image, provide the bounding box for all $<$ref$>$\{prompt\}$<$/ref$>$.\\
$[$refer$]$ please provide the bounding box coordinate of all objects in this sentence describes: $<$ref$>$\{prompt\}$<$/ref$>$\\
$[$refer$]$ can you locate and provide the bounding box for all $<$ref$>$\{prompt\}$<$/ref$>$ in the given image?\\
\textbf{Response:} $<$box$>$\{hbb\}$<$/box$>$\\\\

\textbf{Query for PAL:} \\
$[$refer$]$ give me the dense signal of $<$ref$>$\{prompt\}$<$/ref$>$$<$?$>$\{sparse signal\}$<$/?$>$\\
$[$refer$]$ output the dense signal of the $<$ref$>$\{prompt\}$<$/ref$>$$<$?$>$\{sparse signal\}$<$/?$>$ in the image.\\
$[$refer$]$ from this image, provide the dense signal for $<$ref$>$\{prompt\}$<$/ref$>$$<$?$>$\{sparse signal\}$<$/?$>$.\\
$[$refer$]$ please provide the dense signal coordinate of this region: $<$ref$>$\{prompt\}$<$/ref$>$$<$?$>$\{sparse signal\}$<$/?$>$\\
$[$refer$]$ can you locate and provide the dense signal for $<$ref$>$\{prompt\}$<$/ref$>$$<$?$>$\{sparse signal\}$<$/?$>$ in the given image?\\
\textbf{Response:} $<$?$>$\{dense signal\}$<$/?$>$\\\\

\textbf{Query for GGL (Turn 1):} \\
$[$refer$]$ give me the dense signal of $<$ref$>$\{prompt\}$<$/ref$>$\\
$[$refer$]$ output the dense signal of the $<$ref$>$\{prompt\}$<$/ref$>$ in the image.\\
$[$refer$]$ from this image, provide the dense signal for $<$ref$>$\{prompt\}$<$/ref$>$.\\
$[$refer$]$ please provide the dense signal coordinate of the region this sentence describes: $<$ref$>$\{prompt\}$<$/ref$>$\\
$[$refer$]$ can you locate and provide the dense signal for $<$ref$>$\{prompt\}$<$/ref$>$ in the given image?\\
\textbf{Response:} $<$?$>$\{dense signal\}$<$/?$>$\\
\textbf{Query for GGL (Turn 2):} \\
 The sparse signal corresponding to this dense signal is\\
\textbf{Response:} $<$?$>$\{sparse signal\}$<$/?$>$
\end{mybody}
\captionof{figure}{The instruction fine-tuning template for GeoGround. The placeholder $<$?$>$ can be replaced with $<$box$>$, $<$obb$>$, or $<$seg$>$ depending on the specific situation.}

\label{fig:template}
\end{table*}

\section{Additional Qualitative Results}

See more qualitative results of the REC task in Figs. \ref{fig:viz_hbb_1} and \ref{fig:viz_hbb_2}. See more qualitative results of the REC with OBB task in Figs. \ref{fig:viz_obb_1}, \ref{fig:viz_obb_2} and \ref{fig:viz_obb_3}. See more qualitative results of the RES task in Figs. \ref{fig:viz_seg_1}, \ref{fig:viz_seg_2}, \ref{fig:viz_seg_vlm_1}, \ref{fig:viz_seg_vlm_2} and \ref{fig:viz_seg_vlm_3}.

\begin{figure*}[!t]
\vspace{-0.2cm}
	\begin{center}             % figure uses center environment
        \includegraphics[width=1\linewidth]{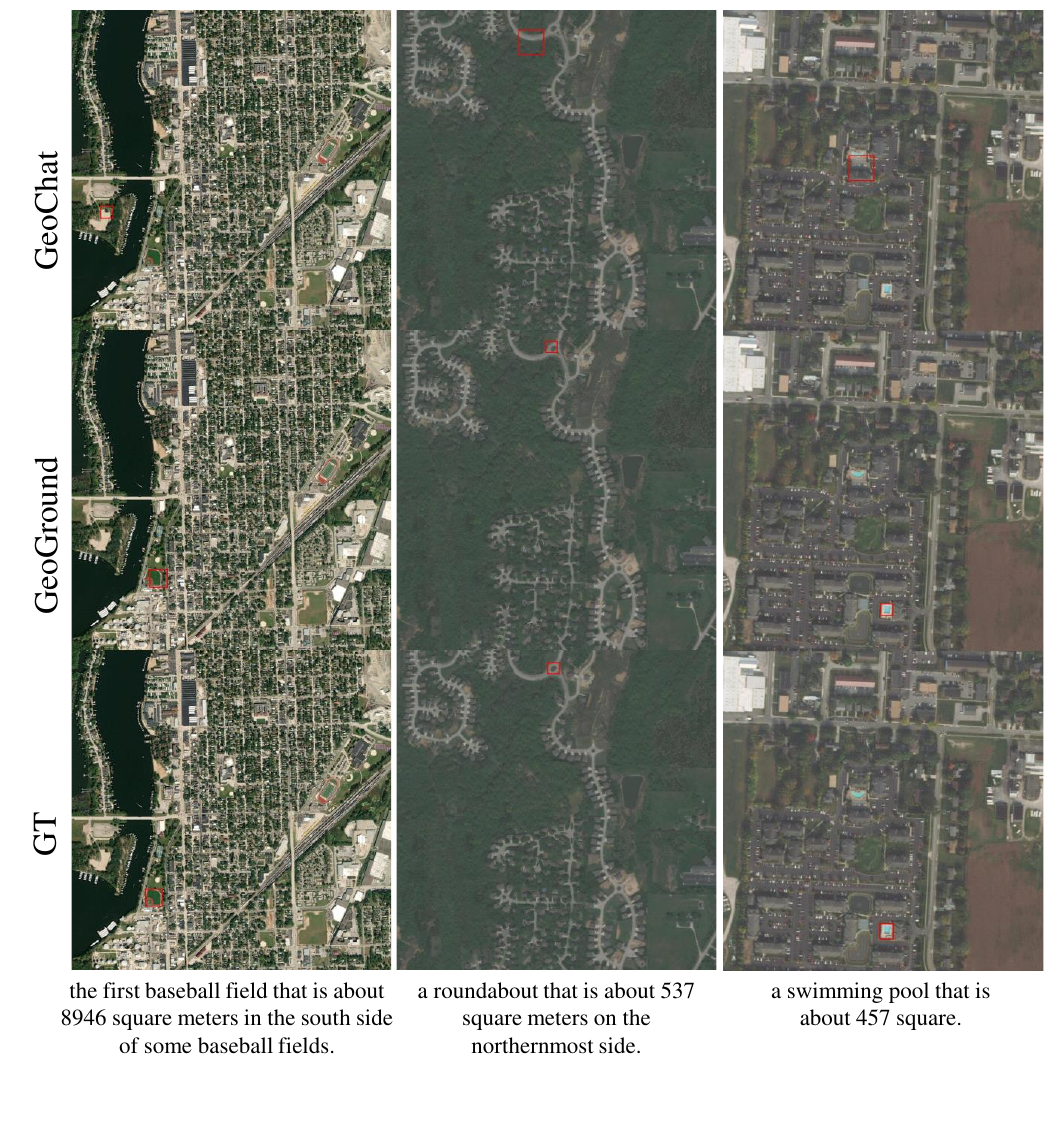}
    \end{center}
\vspace{-1.5cm}
    \caption{Visualizations of GeoGround and GeoChat on RSVG test set with HBB.}
    \label{fig:viz_hbb_1}        
\end{figure*}

\begin{figure*}[!t]
\vspace{-0.2cm}
	\begin{center}             % figure uses center environment
        \includegraphics[width=0.92\linewidth]{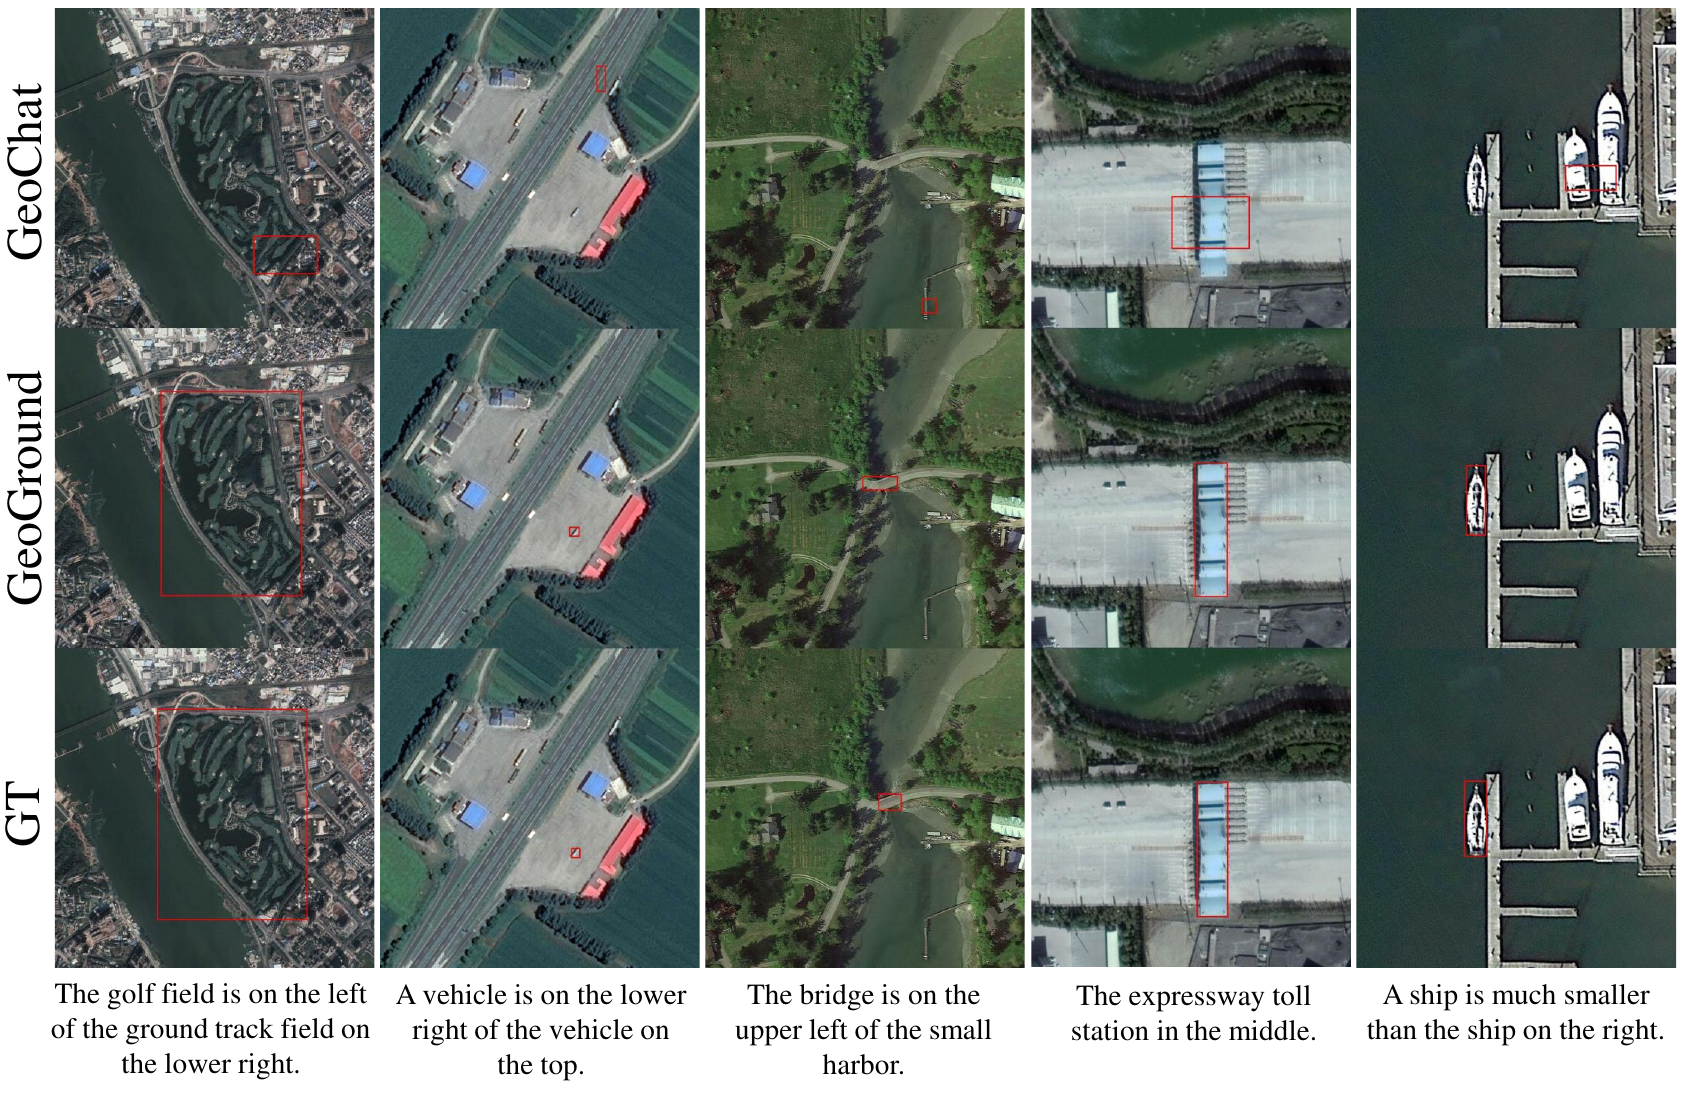}
    \end{center}
\vspace{-0.5cm}
    \caption{Visualizations of GeoGround and GeoChat on DOIR-RSVG test set with HBB.}
    \label{fig:viz_hbb_2}        
\end{figure*}

\begin{figure*}[!t]
\vspace{-0.2cm}
	\begin{center}             % figure uses center environment
        \includegraphics[width=0.92\linewidth]{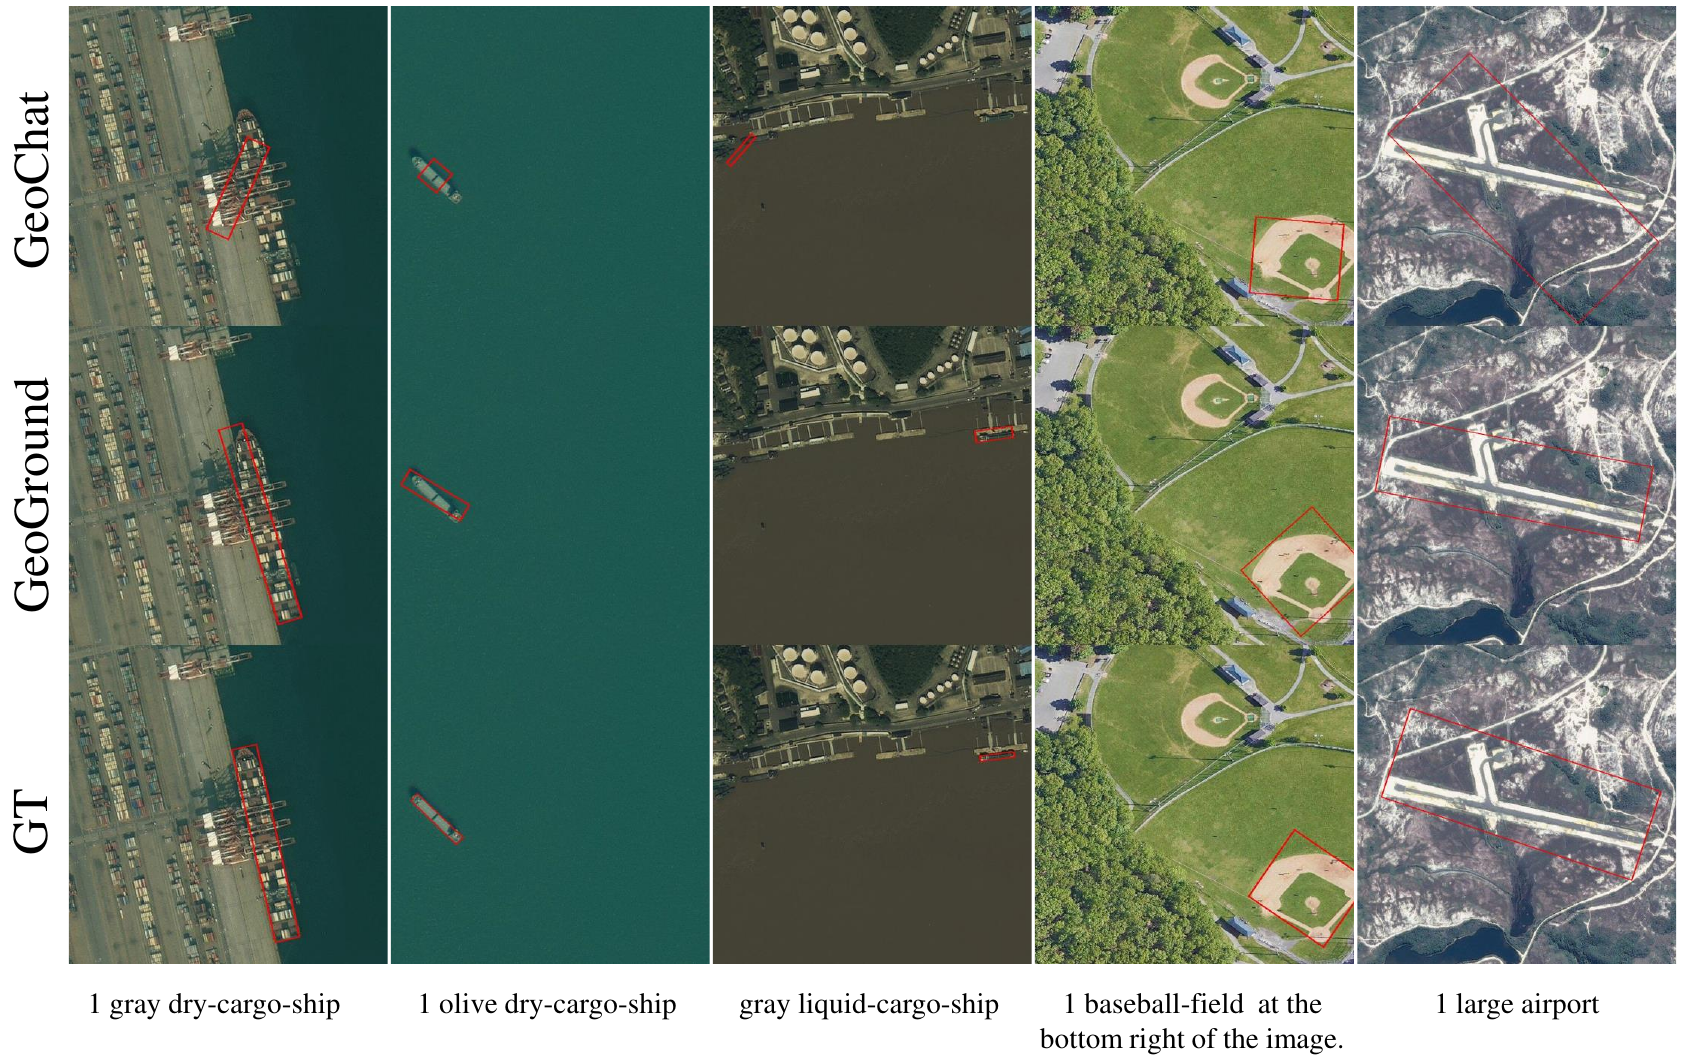}
    \end{center}
\vspace{-0.5cm}
    \caption{Visualizations of GeoGround and GeoChat on GeoChat test set with OBB. Compared to GeoChat, GeoGround, which adopts the le90 angle representation, provides more accurate predictions of the orientation of objects.}
    \label{fig:viz_obb_1}        
\end{figure*}

\begin{figure*}[!t]
\vspace{-0.2cm}
	\begin{center}             % figure uses center environment
        \includegraphics[width=1\linewidth]{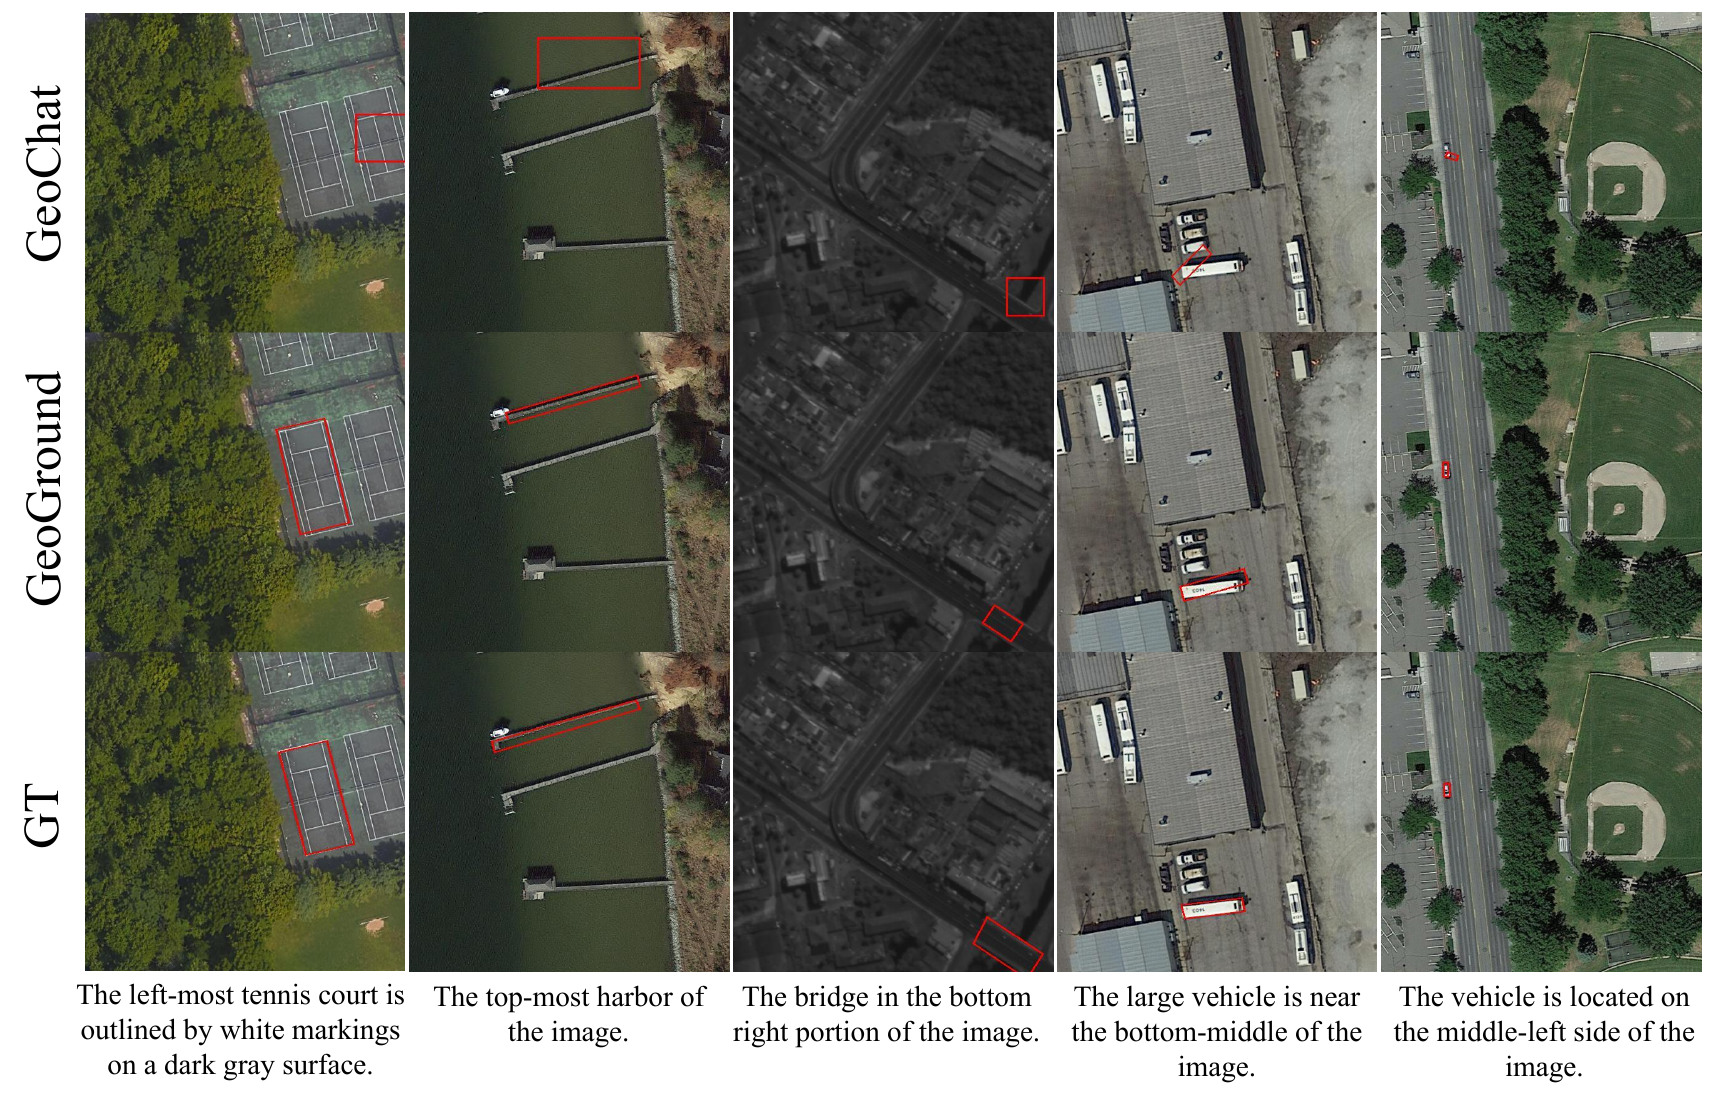}
    \end{center}
\vspace{-0.5cm}
    \caption{Visualizations of GeoGround and GeoChat on VRSBench test set with OBB.}
    \label{fig:viz_obb_2}        
\end{figure*}

\begin{figure*}[!t]
\vspace{-0.2cm}
	\begin{center}             % figure uses center environment
        \includegraphics[width=1\linewidth]{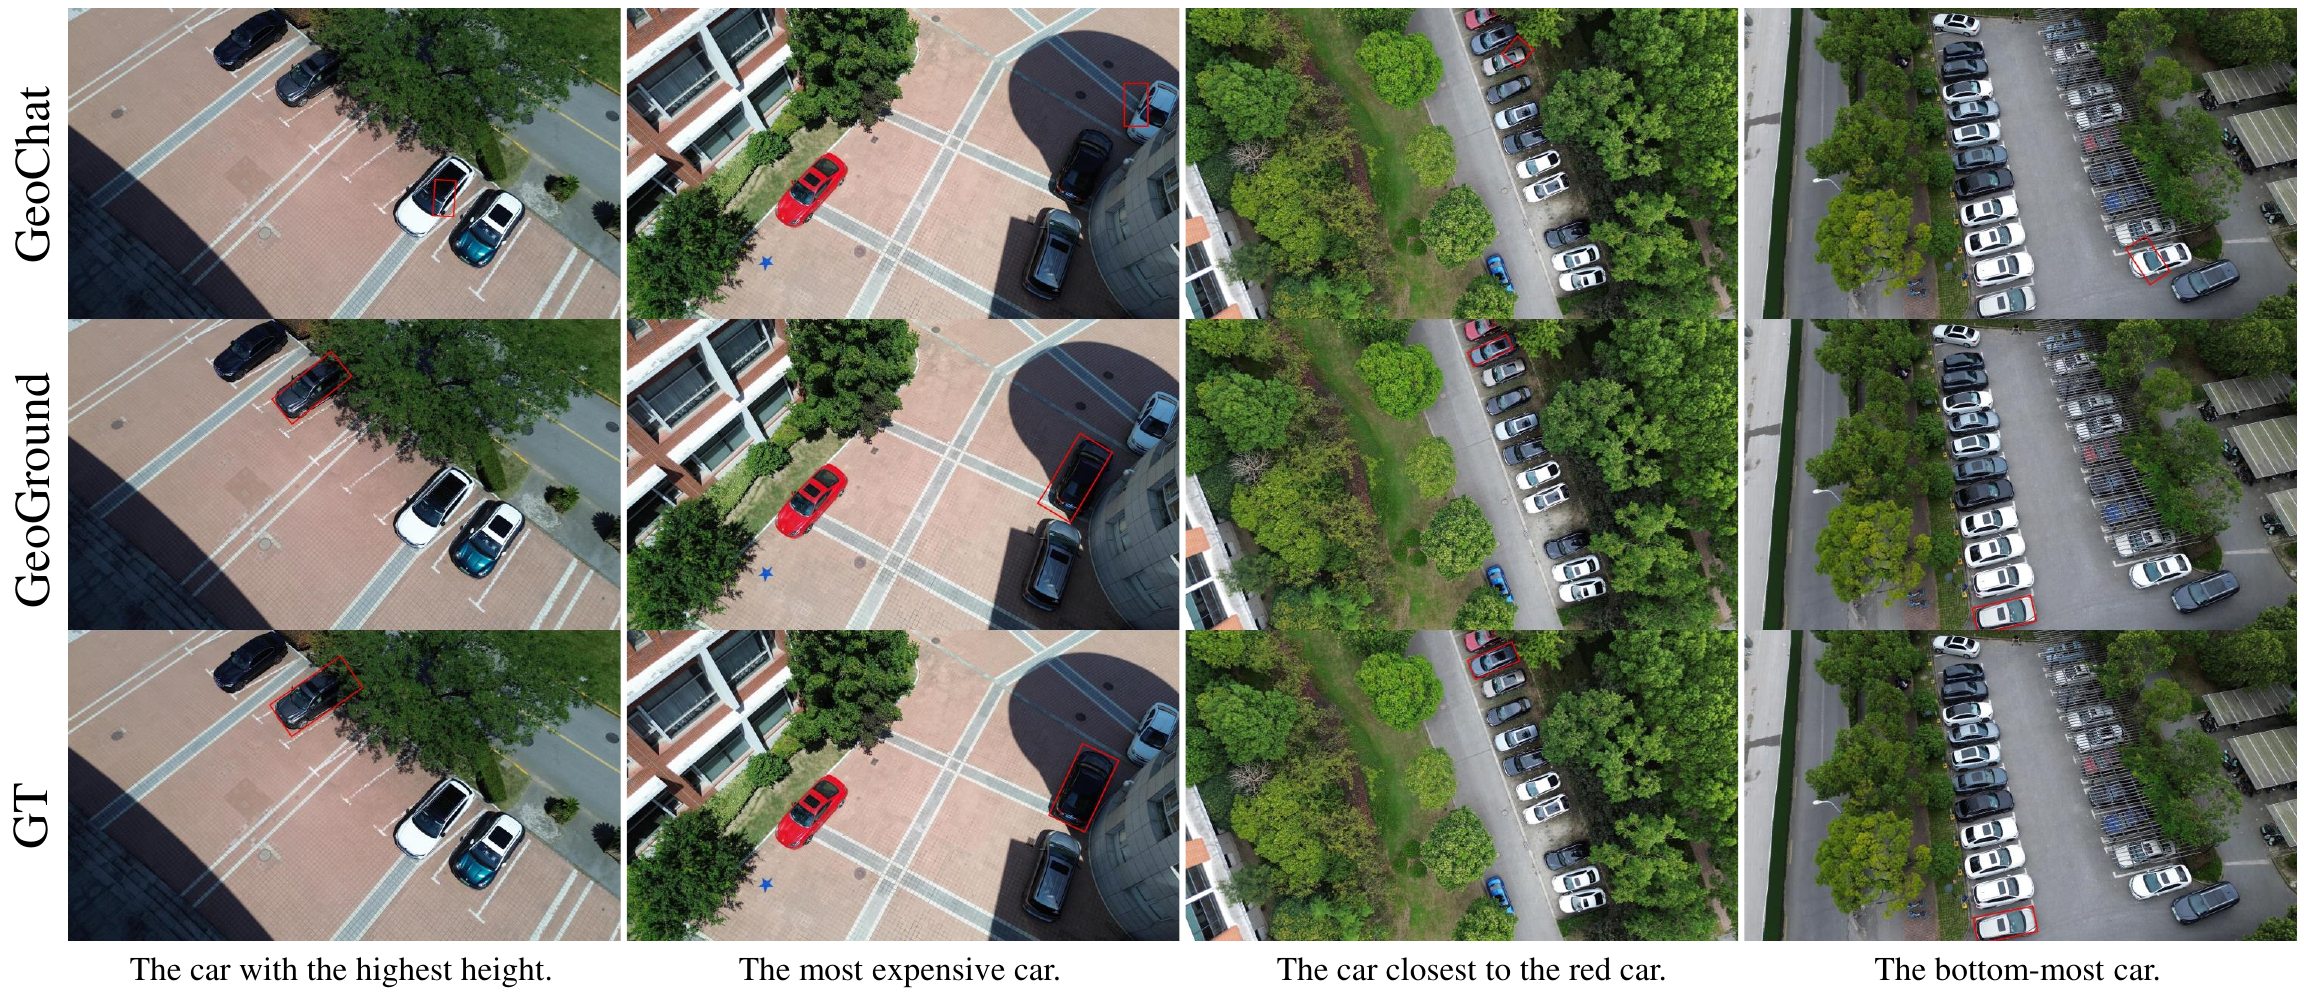}
    \end{center}
\vspace{-0.5cm}
    \caption{Visualizations of GeoGround and GeoChat on AVVG test set with OBB. GeoChat lacks spatial reasoning capabilities and is unable to infer the 3D space from its projection onto the 2D imaging plane.}
    \label{fig:viz_obb_3}        
\end{figure*}

\begin{figure*}[!t]
\vspace{-0.2cm}
	\begin{center}             % figure uses center environment
        \includegraphics[width=1\linewidth]{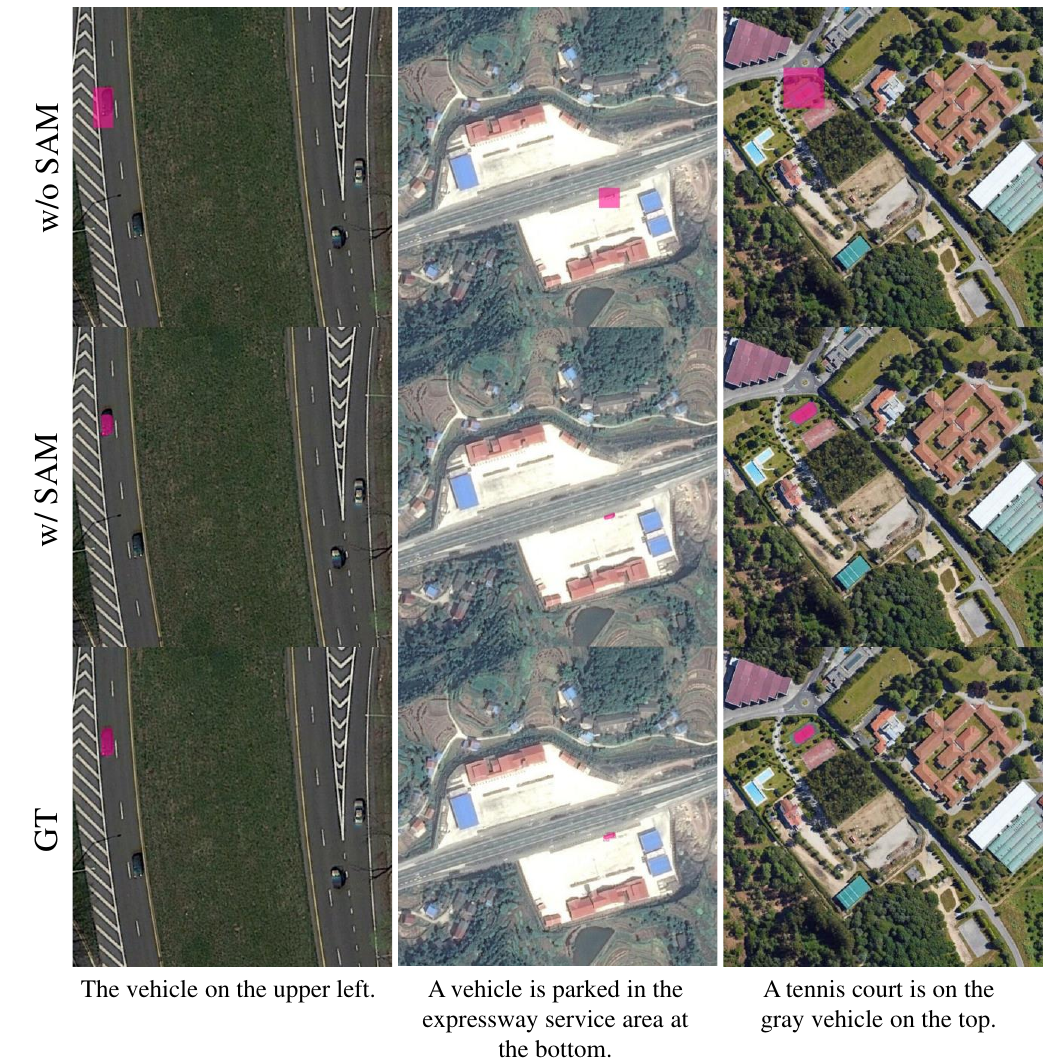}
    \end{center}
\vspace{-0.5cm}
    \caption{Visualization of GeoGround on RRSIS-D for tiny objects, with or without the SAM refiner. For tiny objects, the Matrix4Seg method is currently unable to accurately capture their shapes. Utilizing SAM as a refiner to fine-tune the masks is an effective approach.}
    \label{fig:viz_seg_1}        
\end{figure*}

\begin{figure*}[!t]
\vspace{-0.2cm}
	\begin{center}             % figure uses center environment
        \includegraphics[width=1\linewidth]{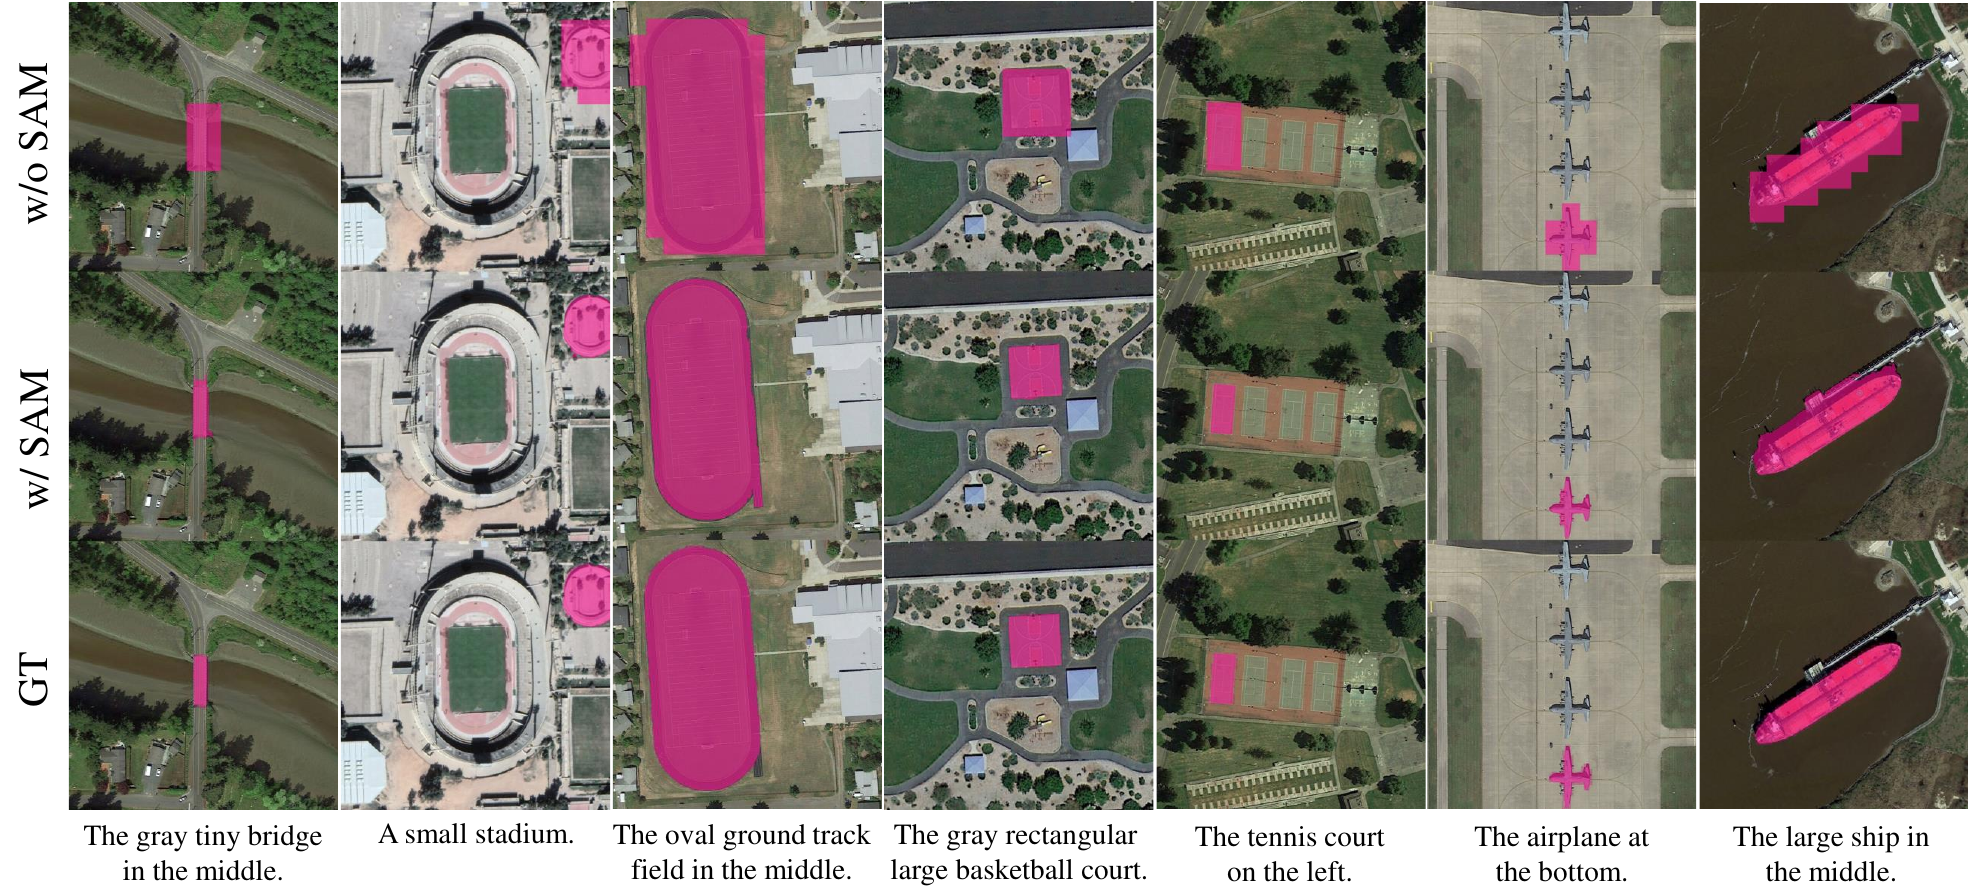}
    \end{center}
\vspace{-0.5cm}
    \caption{Visualizations of GeoGround with and without SAM refiner on the RRSIS-D. The mask refiner can eliminate the mosaic artifacts introduced by Matrix4Seg, further improving the accuracy of the mask.}
    \label{fig:viz_seg_2}        
\end{figure*}

\begin{figure*}[!t]
\vspace{-0.2cm}
	\begin{center}             % figure uses center environment
        \includegraphics[width=1\linewidth]{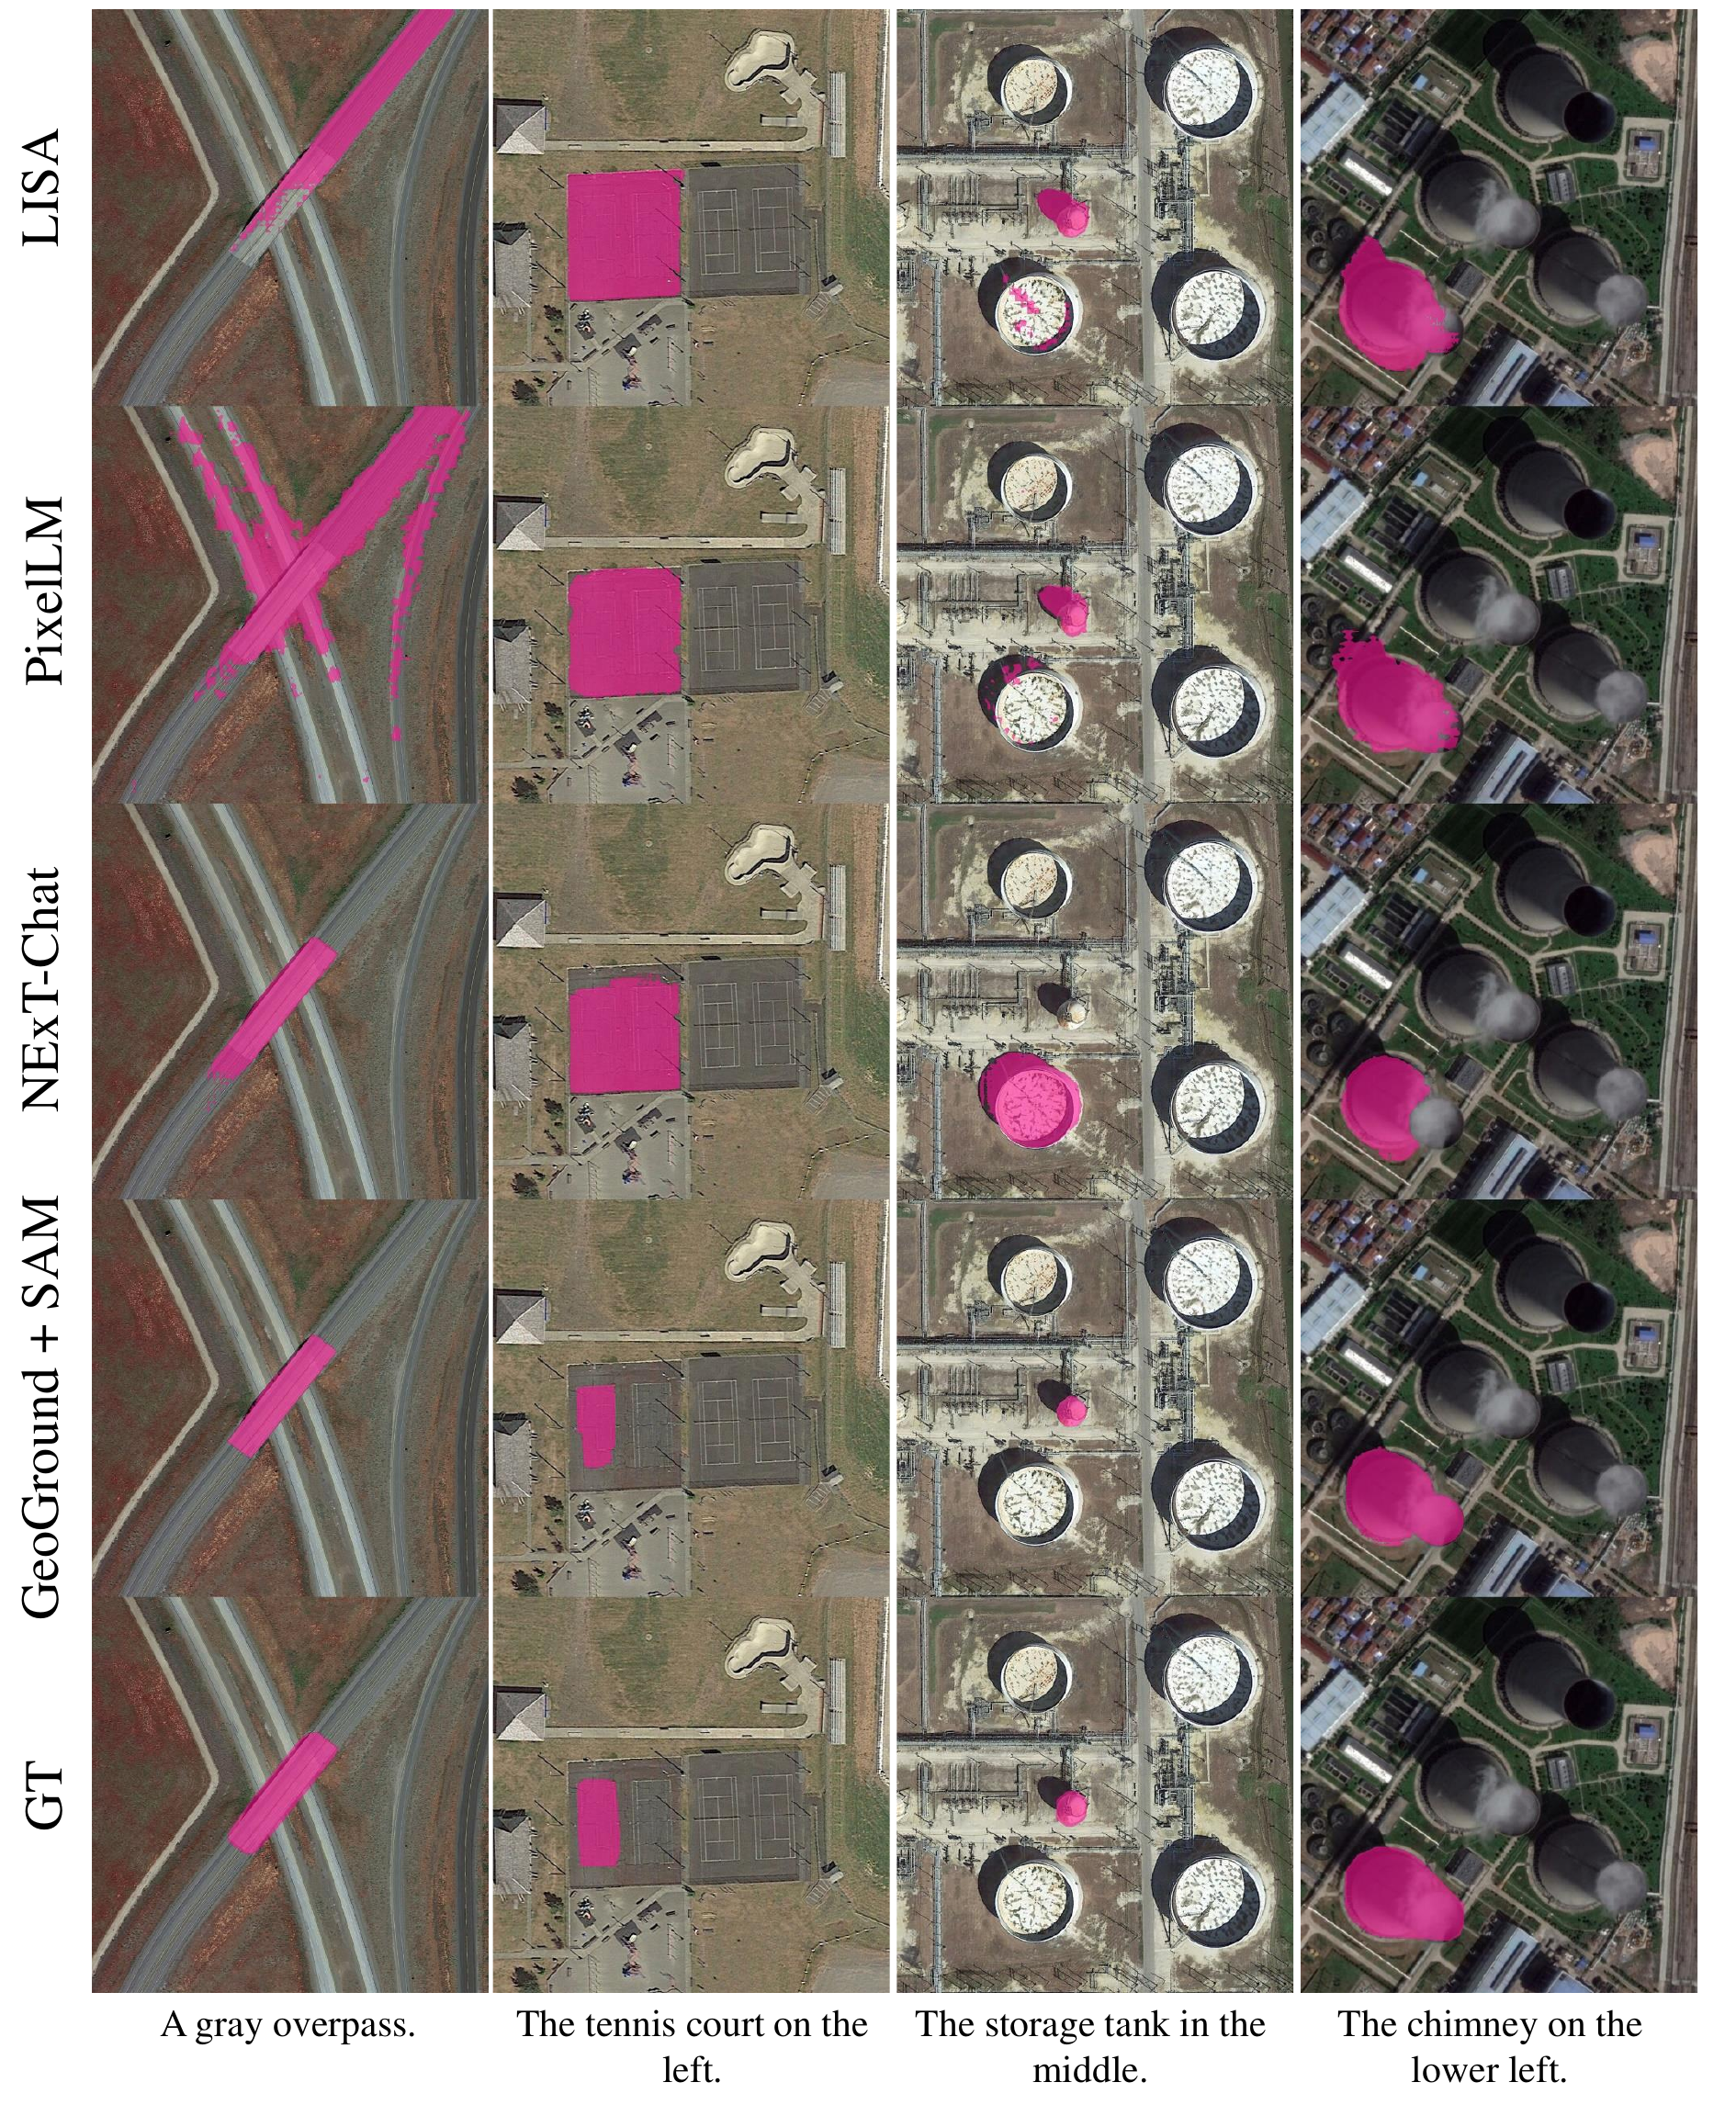}
    \end{center}
\vspace{-0.5cm}
    \caption{Visualizations of GeoGround and other VLMs on the RRSIS-D.}
    \label{fig:viz_seg_vlm_1}        
\end{figure*}

\begin{figure*}[!t]
\vspace{-0.2cm}
	\begin{center}             % figure uses center environment
        \includegraphics[width=1\linewidth]{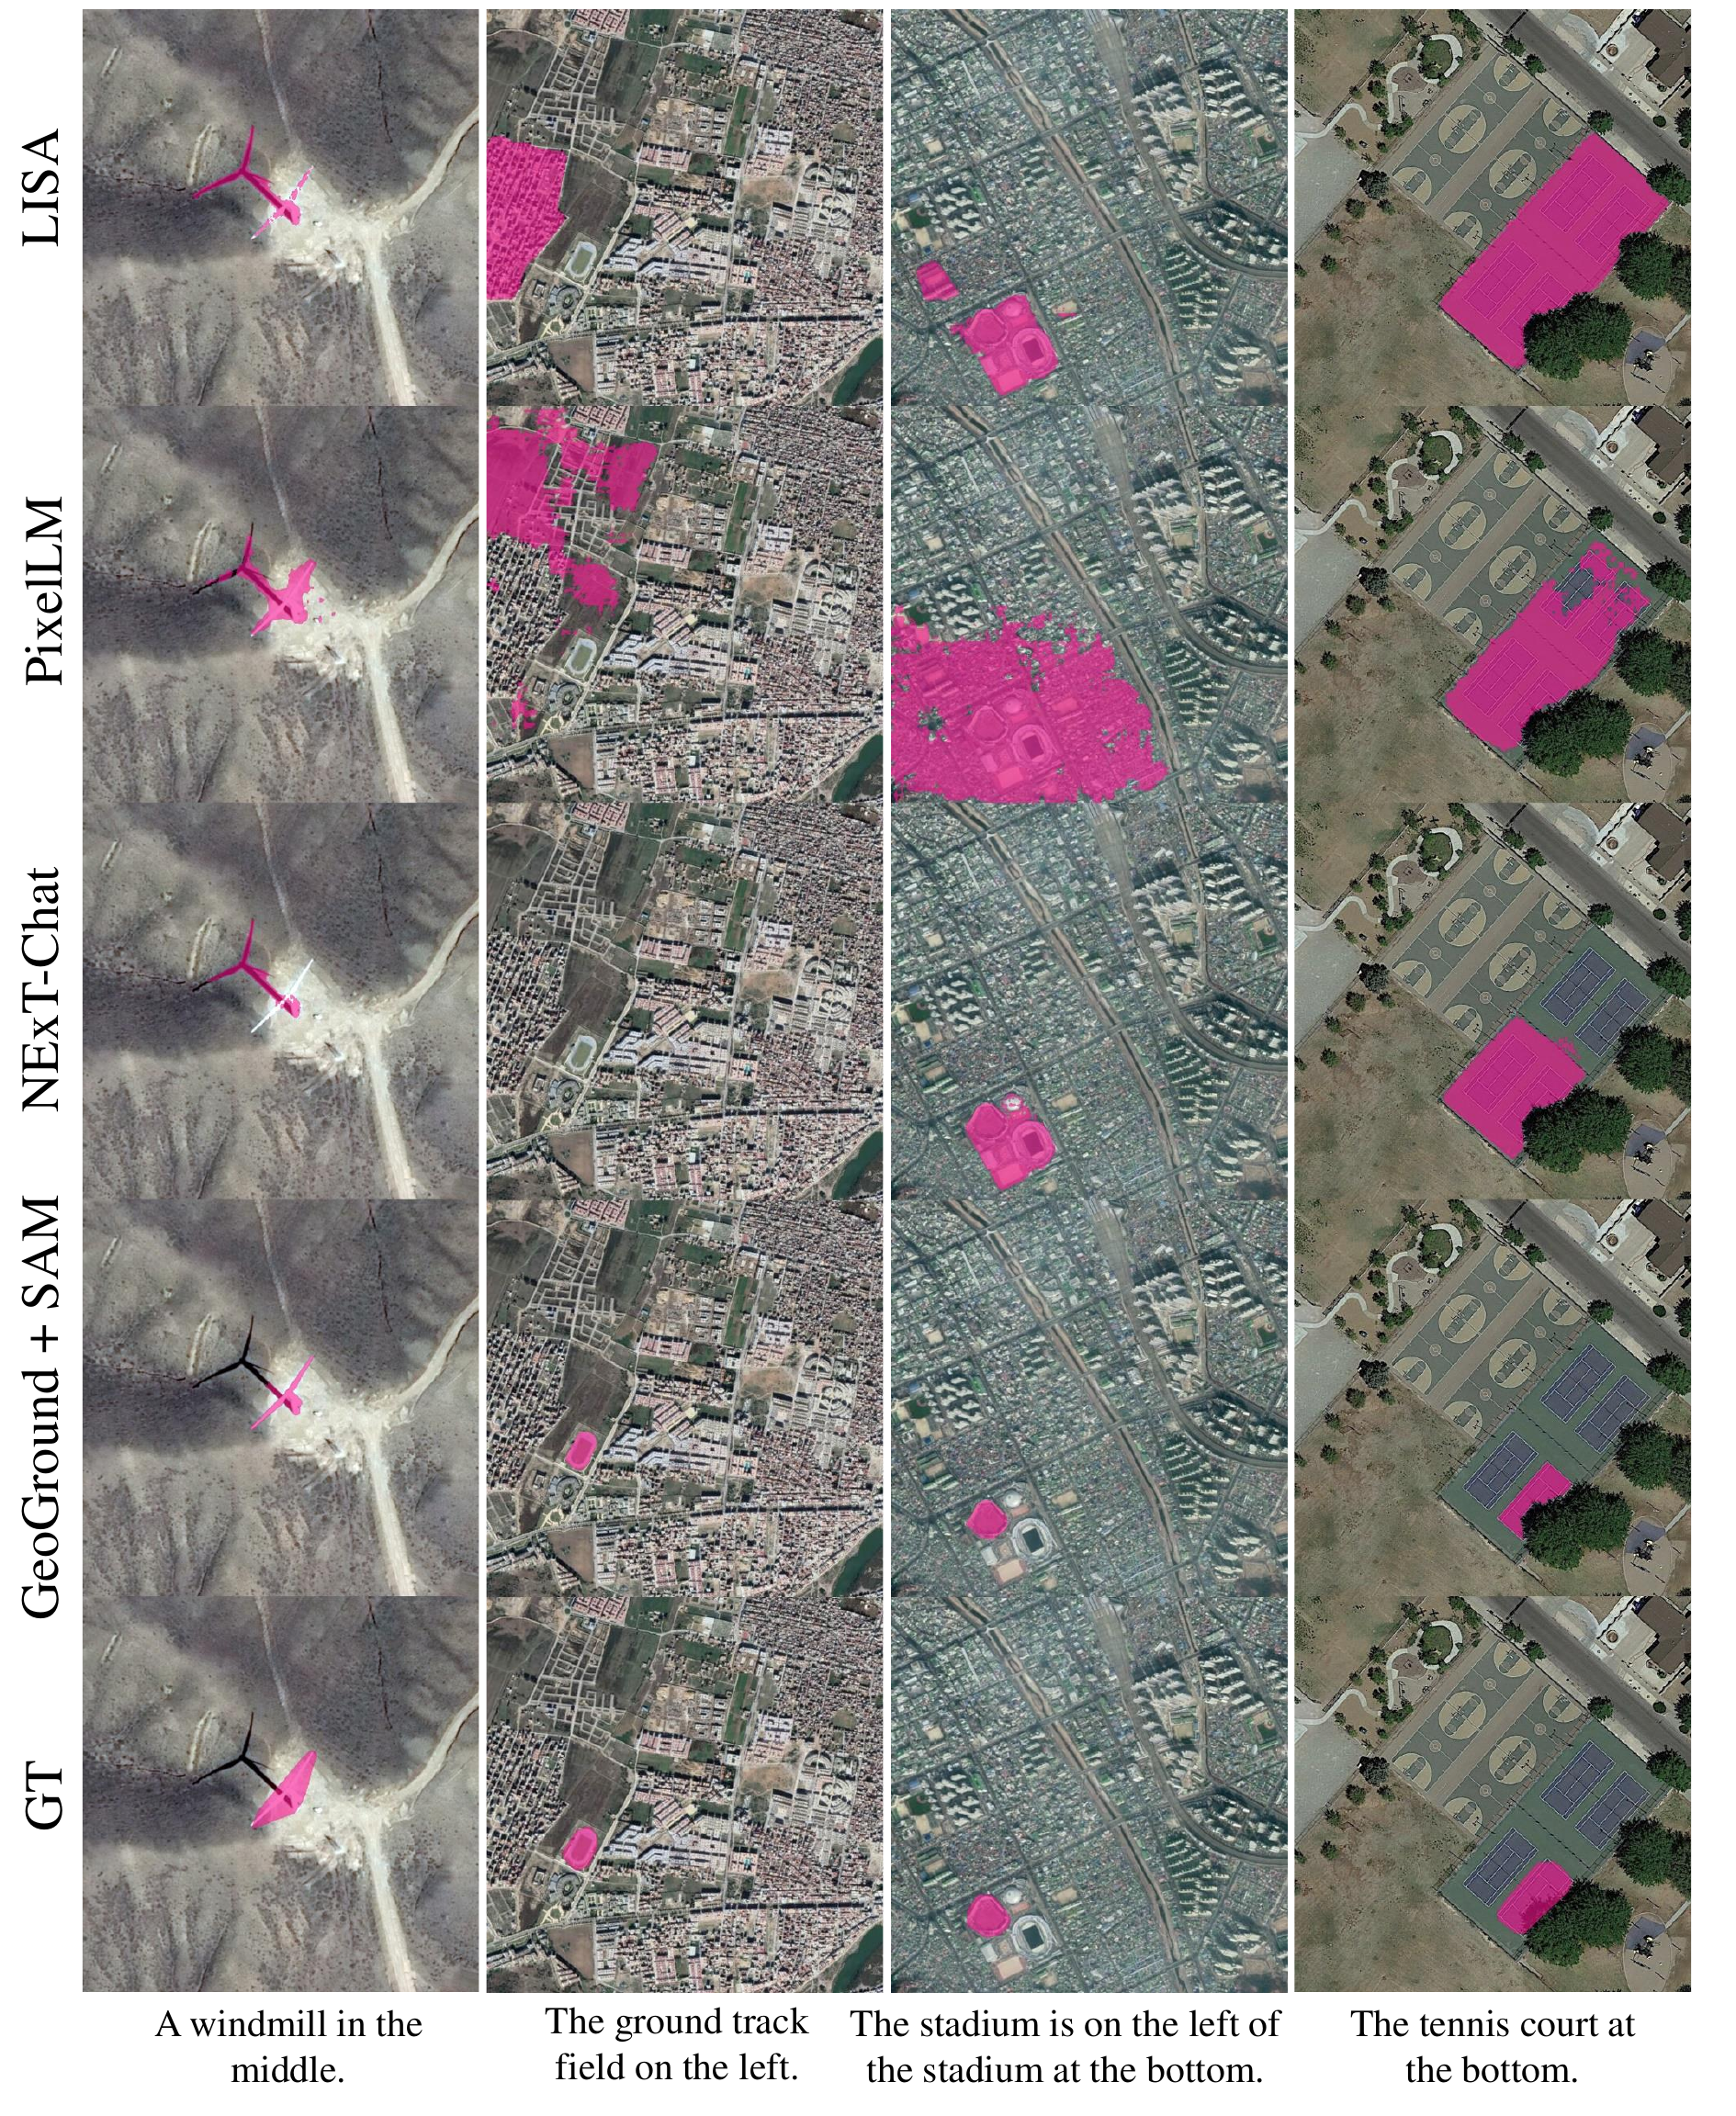}
    \end{center}
\vspace{-0.5cm}
    \caption{Visualizations of GeoGround and other VLMs on the RRSIS-D.}
    \label{fig:viz_seg_vlm_2}        
\end{figure*}

\begin{figure*}[!t]
\vspace{-0.2cm}
	\begin{center}             % figure uses center environment
        \includegraphics[width=1\linewidth]{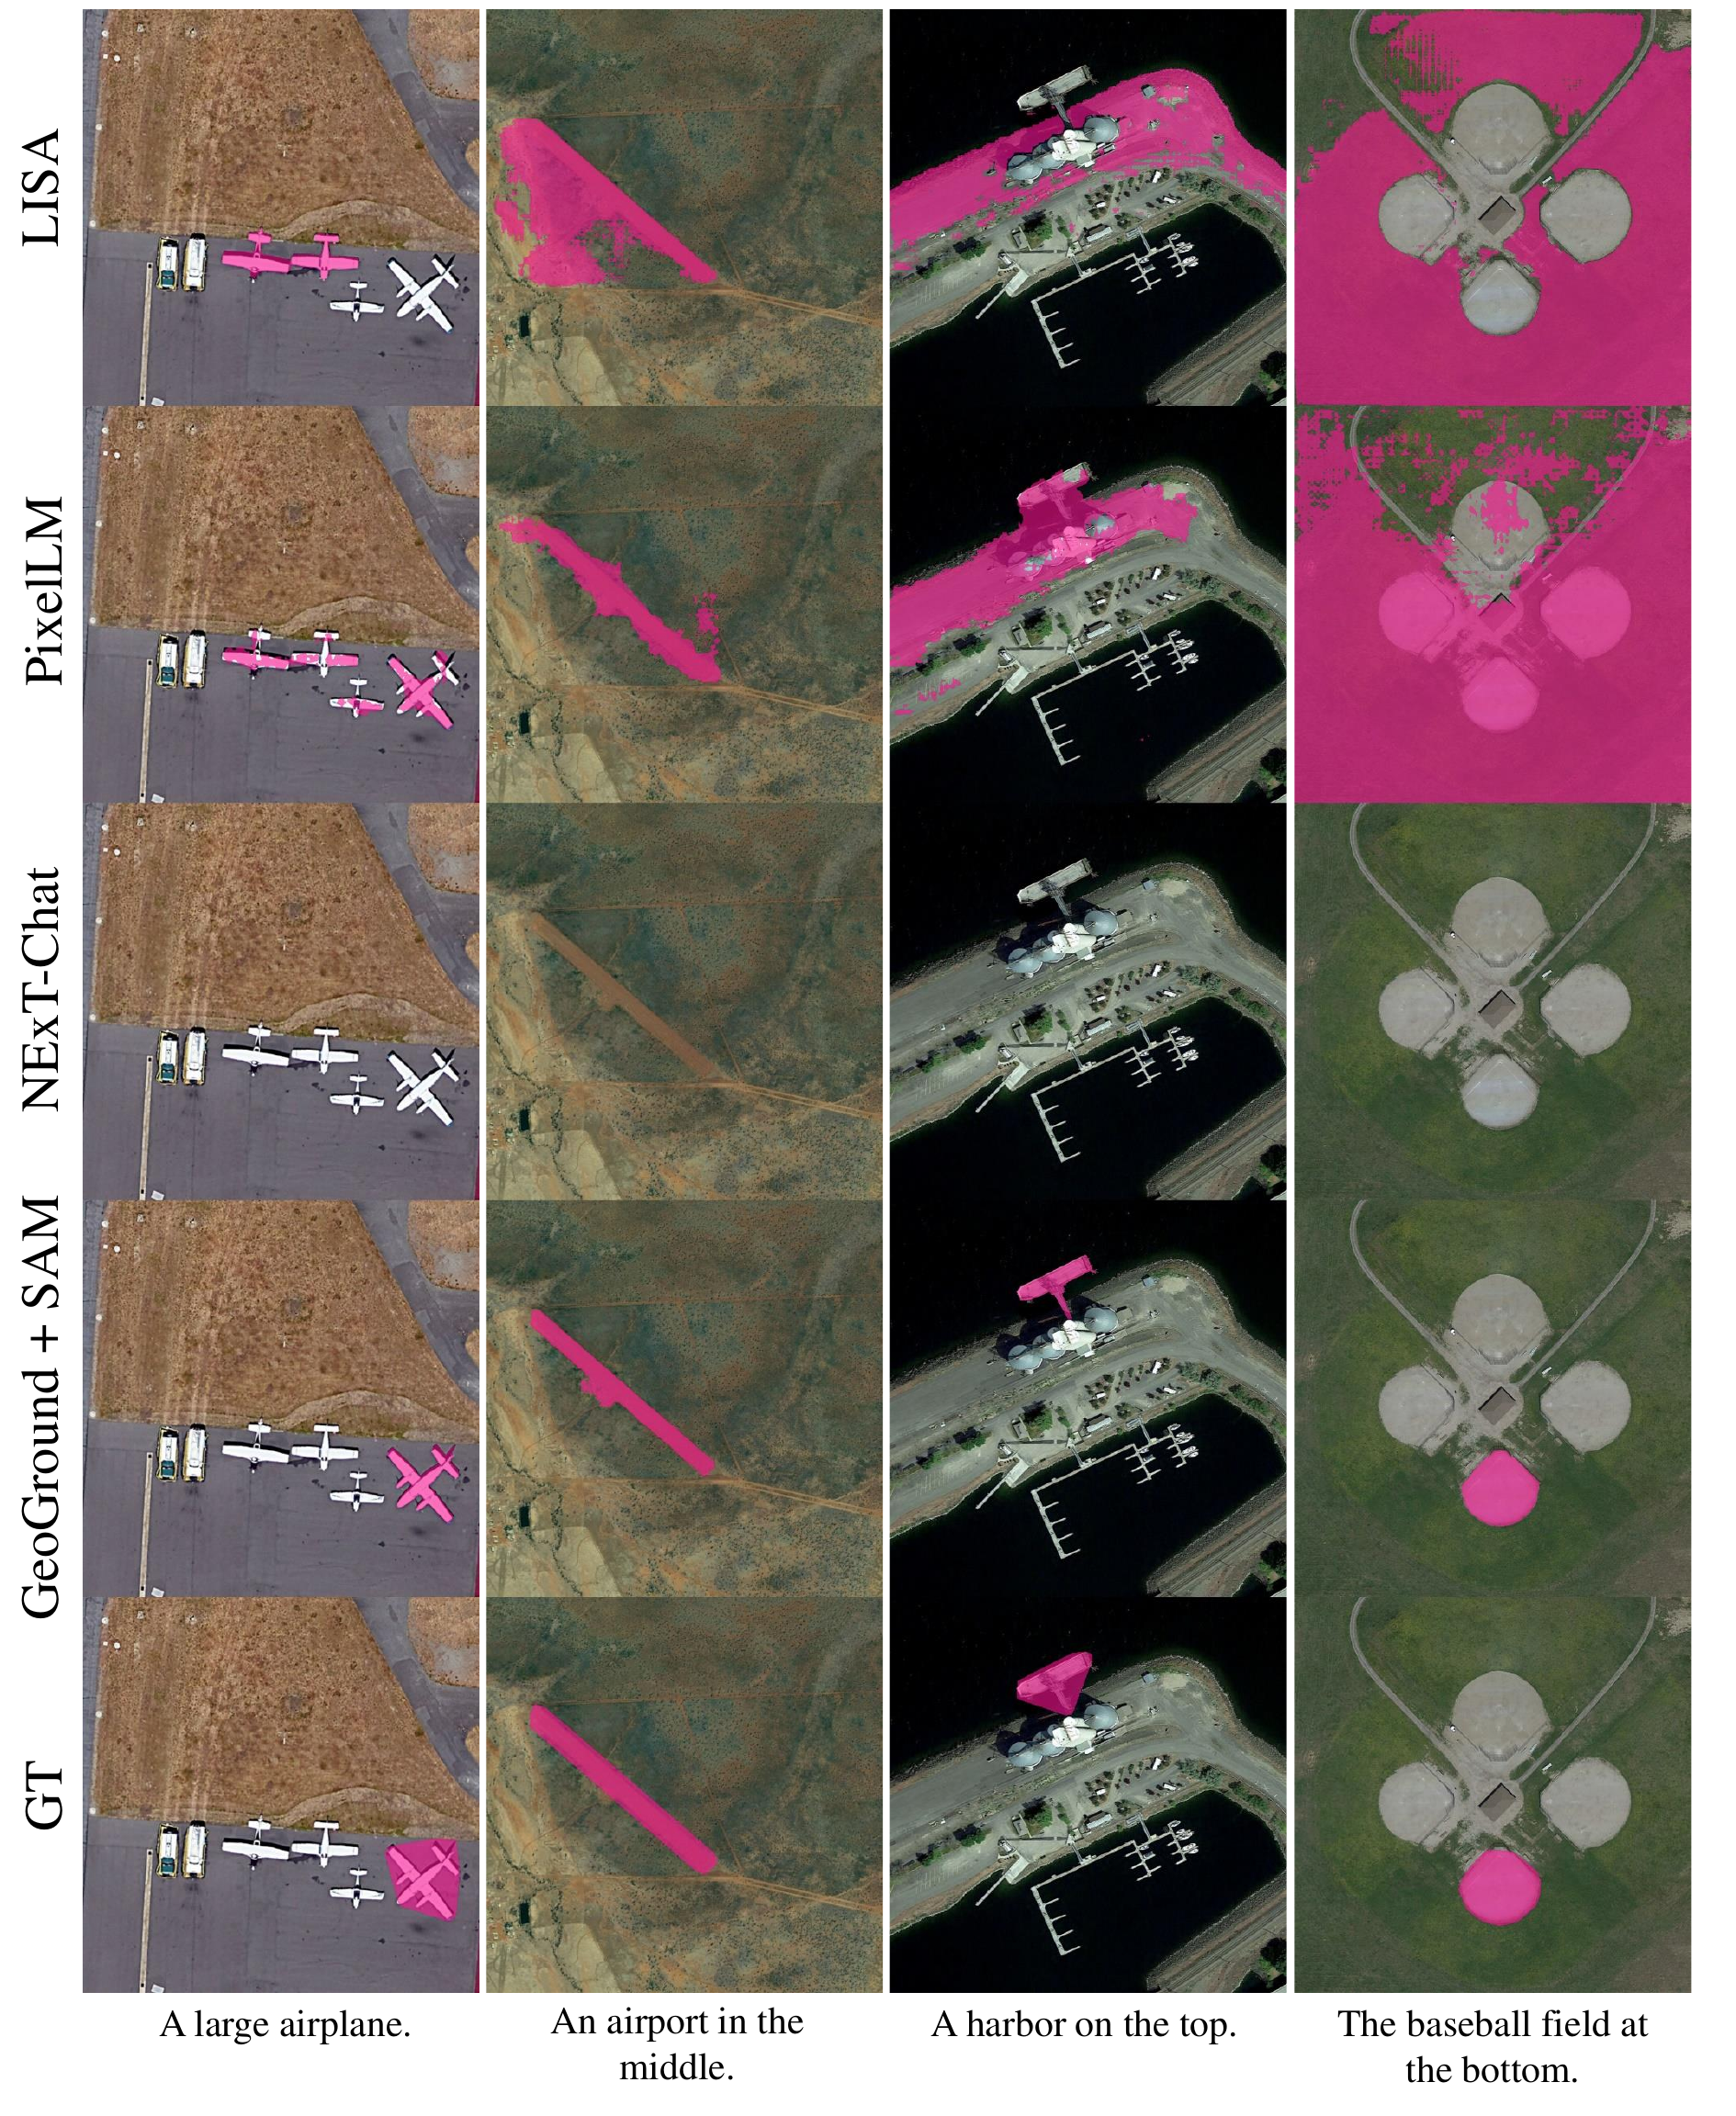}
    \end{center}
\vspace{-0.5cm}
    \caption{Visualizations of GeoGround and other VLMs on the RRSIS-D.}
    \label{fig:viz_seg_vlm_3}        
\end{figure*}
